# Supplementary material for: Emergence of a pseudogap in the BCS-BEC crossover
Source: arXiv:2004.05014 ancillary file (2020-08-11)
Supplement: Supplementary file 1 [file supplemental.pdf]

# Supplemental Material: Emergence of a pseudogap in the BCS–BEC crossover

Adam Richie-Halford,[1,*] Joaquín E. Drut,[2,†] and Aurel Bulgac[1,‡]
[1] Department of Physics, University of Washington, Seattle, Washington 98195–1560, USA
[2] Department of Physics and Astronomy, University of North Carolina, Chapel Hill, North Carolina 27599, USA
(Dated: June 5, 2020)

In these supplemental materials we present mostly technical details of our calculations, including: the model, the auxiliary field quantum Monte Carlo method (with emphasis on constrained ensembles that are not described elsewhere), the finite-size scaling of the condensate fraction, the extrapolations, and other data analysis aspects. In addition, we show results for the Tan contact at finite temperature and away from unitarity which are also novel.

## CONTENTS

I. Model 1

II. AFQMC Method 2
  A. Auxiliary-field quantum Monte Carlo 2
  B. Constrained ensembles 2

III. Tan Contact, $C$ 5

IV. Finite size scaling of the condensate fraction 7

V. Extracting $\Delta$ and $\xi(T)$ from even-odd energy staggering 7

VI. Gaussian process regression of $\xi$ and $\Delta$ 11

VII. Calculating constrained ensemble observables in AFQMC 12
  A. Calculating occupation matrices 12
  B. Calculating the constrained statistical weights 13

VIII. Reducing the number of observable calculations 13

IX. Determining energies for even-odd stagger calculations 13
  A. Extrapolation to the continuum limit 14
  B. Finite range correction 15
  C. Reduced temperature shift 15

References 16

## I. MODEL

The simplest model that exhibits the BCS–BEC crossover has a zero-range, attractive, two-body interaction $V(\mathbf{r}_1 - \mathbf{r}_2) = g\delta(\mathbf{r}_1 - \mathbf{r}_2)$, given by the lattice Hamiltonian

$$\hat{H} = \sum_{\mathbf{k},\sigma\in\{\uparrow,\downarrow\}} \frac{\hbar^2 k^2}{2m} \hat{\psi}^\dagger_\sigma(\mathbf{k})\hat{\psi}_\sigma(\mathbf{k}) - g\sum_{\mathbf{r}} \hat{n}_\uparrow(\mathbf{r})\hat{n}_\downarrow(\mathbf{r}), \quad (1)$$

where $\hat{\psi}^\dagger_\sigma(\mathbf{k}), \hat{\psi}_\sigma(\mathbf{k})$ are the creation and annihilation operators for particles of spin $\sigma$, momentum $\mathbf{k}$ and mass $m$; $g$ is the coupling constant; $V$ is the system volume; and $\hat{n}_\sigma(\mathbf{r}) = \hat{\psi}^\dagger_\sigma(\mathbf{r})\hat{\psi}_\sigma(\mathbf{r})$ is the number density operator at lattice site $\mathbf{r}$.

Following a previous path-integral approach [1, 2], we simulate the system on a cubic lattice of spatial extent $L = N_x\ell$. At unitarity, $N_x \in \{8, 10, 14\}$, while at all other scattering lengths, $N_x \in \{6, 8, 10\}$, with the smallest lattice size being used primarily for determination of critical temperatures from finite-size scaling of the condensate fraction. The lattice constant $\ell$ sets an ultraviolet (UV) momentum cutoff of $k_{\max} = \pi/\ell$, while the lattice size $L$ sets the infrared (IR) cutoff. The lattice coupling constant $g$ is adjusted in order to attain the desired scattering length $a$ [3] using

$$-\frac{1}{g} = \frac{m}{4\pi\hbar^2}\left[\frac{1}{a} - \frac{K_3}{\ell}\right], \quad (2)$$

where $K_3$ is a numerical constant that depends on the choice of single-particle dispersion relation. The first AFQMC studies of the unitary Fermi gas [1] used a parabolic dispersion relation $\epsilon_{\mathbf{k}} = \hbar^2 k/2m$ with a spherical momentum cutoff, $k \leq k_{\max}$, for which $K_3 = 2$. In this paper, we follow later studies that used the same dispersion relation with a cubic momentum cutoff, $|k_i| \leq k_{\max}$, $i \in \{x, y, z\}$ (see e.g. Refs [4, 5]), for which $K_3 \approx 2.442$ [6].

Either choice of cutoff induces a coupling constant-independent effective range, with $r_{\text{eff}} = 4\ell/\pi^2 \approx 0.405\ell$ for the spherical cutoff and $r_{\text{eff}} = \ell\left(12\sqrt{2}/\pi^3\right)\arcsin\left(1/\sqrt{3}\right) \approx 0.337\ell$ for the cubic cutoff. Particle numbers are centered around $N \approx 30$ and we discuss the choice of particle number in Section IX.

* richford@uw.edu
† drut@email.unc.edu
‡ bulgac@uw.edu

## II. AFQMC METHOD

### A. Auxiliary-field quantum Monte Carlo

We summarize our AFQMC method, which is detailed more extensively elsewhere [2], in the case of the grand canonical ensemble (GCE) where the thermodynamic variables are the temperature $T$, the chemical potential $\mu$, and the volume $V$, and the partition function is a trace over a statistical weight that can be interpreted as an imaginary time evolution operator

$$Z = \mathrm{Tr} \exp\left[-\beta\left(\hat{H} - \mu\hat{N}\right)\right], \tag{3}$$

where $\beta = 1/T$. We factor the imaginary time evolution operator using a Suzuki-Trotter expansion [7, 8]

$$\begin{aligned}\exp\left[-\beta\left(\hat{H}-\mu\hat{N}\right)\right] &= \exp\left[-\frac{\tau\left(\hat{K}-\mu\hat{N}\right)}{2}\right] \\ &\times \left\{\prod_{j=1}^{N_\tau} \exp\left(-\tau\hat{V}\right)\exp\left[-\tau\left(\hat{K}-\mu\hat{N}\right)\right]\right\} \\ &\times \exp\left[+\frac{\tau\left(\hat{K}-\mu\hat{N}\right)}{2}\right] + \mathcal{O}\left(\tau^2\right),\end{aligned} \tag{4}$$

where the inverse temperature has been decomposed into a temporal lattice with spacing $\tau$: $\beta = N_\tau \tau$. The two-body interaction term

$$\exp\left[-\tau\hat{V}\right] = \exp\left[g\tau\ell^3\sum_{\mathbf{r}}\hat{n}_\uparrow(\mathbf{r})\hat{n}_\downarrow(\mathbf{r})\right] \tag{5}$$

is then represented using a discrete Hubbard-Stratonovich transformation [9–11]:

$$\begin{aligned}\exp\left[g\tau\hat{n}_\uparrow(\mathbf{r})\hat{n}_\downarrow(\mathbf{r})\right] = \frac{1}{2}\sum_{\sigma(\mathbf{r},\tau_j)=\pm1}&\left[1 + A\sigma(\mathbf{r},\tau_j)\hat{n}_\uparrow(\mathbf{r})\right] \\ &\times\left[1 + A\sigma(\mathbf{r},\tau_j)\hat{n}_\downarrow(\mathbf{r})\right],\end{aligned} \tag{6}$$

where $A = \sqrt{\exp(g\tau) - 1}$, and $\sigma(\mathbf{r}, \tau_j)$ is an auxiliary field that can take the value $\pm1$ at each point on the spacetime lattice given by the vectors $\mathbf{r}$ and time slices $\tau_j$. The partition function can then be represented as an integral over the auxiliary fields

$$Z = \int \mathcal{D}\sigma\left(\mathbf{r},\tau_j\right)\mathrm{Tr}\,\hat{\mathcal{U}}[\sigma] \tag{7}$$

where $\hat{\mathcal{U}}$ is the decomposed statistical weight in Eq. (4). The statistical weight can be expressed as a product of spin-up and spin-down operators

$$\hat{\mathcal{U}}[\sigma] = \hat{\mathcal{U}}_\uparrow[\sigma]\hat{\mathcal{U}}_\downarrow[\sigma], \quad \text{where} \quad \hat{\mathcal{U}}_\uparrow[\sigma] = \hat{\mathcal{U}}_\downarrow[\sigma] \quad \text{if} \quad \mu_\uparrow = \mu_\downarrow. \tag{8}$$

The expectation value of an observable is

$$\langle\mathcal{O}\rangle = \frac{\mathrm{Tr}\,\hat{\mathcal{O}}\hat{\mathcal{U}}}{\mathrm{Tr}\,\hat{\mathcal{U}}[\sigma]} = \int\mathcal{D}\sigma\frac{\mathrm{Tr}\,\hat{\mathcal{U}}[\sigma]}{Z}\frac{\mathrm{Tr}\,\hat{\mathcal{O}}\hat{\mathcal{U}}[\sigma]}{\mathrm{Tr}\,\hat{\mathcal{U}}[\sigma]}. \tag{9}$$

When we use $\mathcal{U}[\sigma]$ to represent $\hat{\mathcal{U}}[\sigma]$ in the single particle Hilbert space using a plane-wave basis, we get

$$\begin{aligned}\mathrm{Tr}\,\hat{\mathcal{U}}[\sigma] &= \det\left[1 + \mathcal{U}[\sigma]\right] &\text{(10a)}\\ &= \det\left[1+\mathcal{U}_\uparrow[\sigma]\right]\det\left[1+\mathcal{U}_\downarrow[\sigma]\right] &\text{(10b)}\\ &= \det{}^2\left[1+\mathcal{U}_\uparrow[\sigma]\right], &\text{(10c)}\end{aligned}$$

with the last equality holding when $\mu_\uparrow = \mu_\downarrow$, in which case $\mathrm{Tr}\,\hat{\mathcal{U}}$ becomes a positive definite probability measure for our AFQMC calculations

$$\begin{aligned}P[\sigma] &= \frac{\det^2\left[1+\mathcal{U}_\uparrow[\sigma]\right]}{Z} &\text{(11a)}\\ &= \frac{1}{Z}\exp\left(2\,\mathrm{Tr}\log\left[1+\mathcal{U}_\uparrow[\sigma]\right]\right) &\text{(11b)}\end{aligned}$$

and

$$\left\langle\hat{\mathcal{O}}\right\rangle = \sum_\sigma P[\sigma]\frac{\mathrm{Tr}\,\hat{\mathcal{O}}\hat{\mathcal{U}}[\sigma]}{\det\left[1+\mathcal{U}[\sigma]\right].} \tag{11c}$$

The one-body density matrix is represented in position space

$$n(\mathbf{r}_1,\mathbf{r}_2,\sigma) = \left[\frac{\mathcal{U}[\sigma]}{1+\mathcal{U}[\sigma]}\right]_{\mathbf{r}_1,\mathbf{r}_2}, \tag{12}$$

with an analogous representation calculated in momentum space by Fourier transform.

As suggested in Eq. (11c), because the auxiliary fields $\sigma$ are discrete, the integration over auxiliary fields is actually a summation over all $2^{N_x N_y N_z N_\tau}$ possible field configurations, necessitating the use of Monte Carlo integration with the standard Metropolis algorithm [12, 13].

When the number of imaginary time slices $N_\tau$ grows large, the matrix product $\mathcal{U}$ becomes numerically unstable. Departing from our previous calculations, we stabilize $\mathcal{U}$ using *QDR* decomposition as opposed to singular value decomposition [14], as shown in Section VII.

All of our results were computed using non-parametric bootstrap sampling to account for covariance of observables that depend on both the energy and the particle number (e.g. the energy in units of the Fermi energy) and we have omitted points which failed to meet our convergence criterion of a Gelman-Rubin diagnostic [15, 16] of $R_c \leq 1.1$ for GCE observables and $R_c \leq 1.2$ for the projected observables described in the next section.

### B. Constrained ensembles

The method explained in Section II A was described in the context of the grand canonical ensemble (GCE).

However, calculations of the observables $\Delta_E$ and $\chi_s$ require simulation at fixed particle number or fixed particle asymmetry in the canonical ensemble. A similar problem is encountered in nuclear physics when one wants to simulate nuclei with fixed neutron and proton numbers. One approach is to constrain the GCE using particle projection methods [17–21].

In the following sections, we present the formalism for constraining the GCE, but first we sketch the main idea of particle projection and the novelty of our particle asymmetry projection. Previous studies have constrained the number of spin-up particle, $N_\uparrow$, spin-down particles, $N_\downarrow$, or the total particle number $N_+ \equiv N_\uparrow + N_\downarrow$, by simultaneous projection of both $N_\uparrow$ and $N_\downarrow$. This is represented schematically in Fig. 1, where the shaded blob represents the distribution of some statistical weight in the GCE over particle numbers $N_\uparrow$ and $N_\downarrow$. Constraining the GCE to a single flavor particle number, either $N_\uparrow$ or $N_\downarrow$, can be interpreted as projecting the GCE distribution onto a single slice along either axis. And constraining the GCE to a specific pair $(N_\uparrow, N_\downarrow)$ may be viewed as simultaneous projection along both axes to collapse onto a target point, which may be some distance away from the thermal average in the GCE. If instead, one wishes to constrain the total particle number only, then one projects onto the diagonal line with slope one.

In this work, we introduce another constrained ensemble using particle number asymmetry projection, represented in Fig. 1 by the diagonal line with negative slope representing a constant value of $N_- \equiv N_\uparrow - N_\downarrow$. If one wishes to constrain the GCE to a specific pair, then one can choose $(N_+, N_-)$ to achieve the equivalent $(N_\uparrow, N_\downarrow)$ pair, rotating the projection axes by $\pi/4$ radians. But this choice of rotation is not arbitrary; it is (a) physically motivated, (b) chosen to minimize variance in one direction, and (c) lacks a sign problem when implemented in AFQMC. Firstly (a), it is appropriate to constrain only the particle number asymmetry to measure some observables, as is the case when measuring spin susceptibility. Secondly (b), the statistical weights in the GCE are often sharply peaked along the $N_-$ axis, falling off more quickly in the $N_-$ direction than in the $N_+$ direction, such that this specific choice of projection axes minimizes the variance on one of the axes. Lastly (c), as we will show in Section II B 2, when implemented using AFQMC methods, this asymmetry projection lacks a sign problem. To our knowledge, no other constrained ensemble studies have used the asymmetry projection method.

Lastly, before we formally introduce the projection methods, we should note that in reality, the statistical weights depicted in Fig. 1 are not simply concave as shown in the figure. Rather, they have an "egg carton" shape to account for the impossibility of having even values of $N_+$ with odd values of $N_-$ and vice versa.

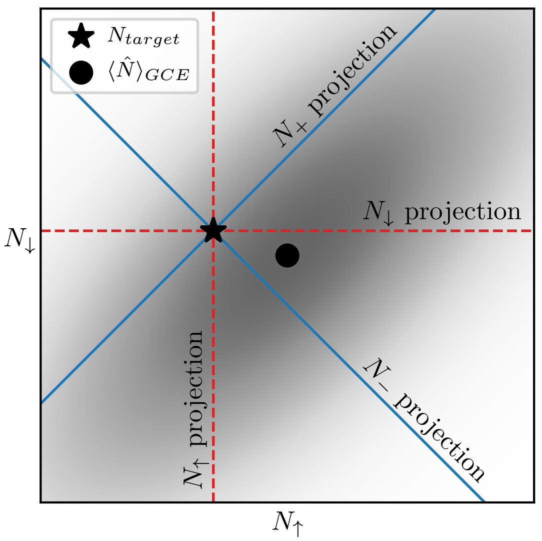


FIG. 1. Schematic representation of various GCE projection methods. The GCE statistical weight is represented as a shaded blob which is broadly distributed in the $N_+$ direction and sharply peaked in the $N_-$ direction. Single spin number projection is represented by the red dashed lines parallel to the $N_\uparrow$ and $N_\downarrow$ axes. Total particle number and particle number asymmetry projection are represented by the blue solid lines.

### *1. Projecting particle number for single flavor fermions*

To constrain the particle number in simulations of single flavor fermions we introduce a slight generalization of the partition function and of the expectation values:

$$\mathcal{Y}(\varphi) = \exp\left[-\beta\left(\hat{H} - \mu\hat{N}\right) - i\varphi\left(\hat{N} - N\right)\right], \tag{13a}$$

$$\mathcal{Z}(\varphi) = \frac{1}{Z}\,\mathrm{Tr}\left[\mathcal{Y}(\varphi)\right] = \left\langle \exp\left[-i\varphi\left(\hat{N} - N\right)\right]\right\rangle, \tag{13b}$$

$$\mathcal{E}(\varphi) = \frac{\mathrm{Tr}\left[\hat{H}\mathcal{Y}(\varphi)\right]}{Z} = \left\langle \hat{H}\exp\left[-i\varphi(\hat{N} - N)\right]\right\rangle, \tag{13c}$$

$$\mathcal{N}(\varphi) = \frac{\mathrm{Tr}\left[\hat{N}\mathcal{Y}(\varphi)\right]}{Z} = \left\langle \hat{N}\exp\left[-i\varphi(\hat{N} - N)\right]\right\rangle, \tag{13d}$$

where

$$Z = \mathrm{Tr}\exp\left[-\beta\left(\hat{H} - \mu\hat{N}\right)\right], \tag{13e}$$

as in the GCE and the angle brackets signify the usual GCE expectation value. The additional phase factor $\exp(iN\varphi)$, where $N$

$$N = \left\langle \hat{N} \right\rangle = \frac{1}{Z}\,\mathrm{Tr}\left[\hat{N}\exp\left[-\beta(\hat{H} - \mu\hat{N})\right]\right], \tag{14}$$

cancels the highly oscillatory character of these functions and renders them very smooth. Moreover, as numerical

calculations show, the imaginary parts of $\mathcal{Z}(\varphi)$, $\mathcal{E}(\varphi)$, and $\mathcal{N}(\varphi)$ are small [21]. Without the additional phase factor $\exp(iN\varphi)$ these functions are periodic functions of $\varphi$, with the period $2\pi$. They also satisfy the relations:

$$\mathcal{Z}(\varphi) = \mathcal{Z}^*(-\varphi), \tag{15a}$$
$$\mathcal{E}(\varphi) = \mathcal{E}^*(-\varphi), \tag{15b}$$
$$\mathcal{N}(\varphi) = \mathcal{N}^*(-\varphi). \tag{15c}$$

Using these relations one can now introduce the projected particle number probability distribution in the grand canonical ensemble and the particle projected expectation values

$$P(\nu) = \int_0^\pi \frac{d\varphi}{\pi} \mathcal{Z}(\varphi) \exp[i(\nu - N)\varphi], \tag{16a}$$
$$E_p(\nu) = \frac{1}{P(\nu)} \int_0^\pi \frac{d\varphi}{\pi} \exp[i(\nu - N)\varphi]\mathcal{E}(\varphi), \tag{16b}$$
$$N_p(\nu) = \frac{1}{P(\nu)} \int_o^\pi \frac{d\varphi}{\pi} \exp[i(\nu - N)\varphi]\mathcal{N}(\varphi), \tag{16c}$$

where $\nu$ is an integer argument and

$$P(\nu) = \frac{1}{Z} \mathrm{Tr} \left[\delta_{\nu,\hat{N}} \exp\left[-\beta\left(\hat{H} - \mu\hat{N}\right)\right]\right], \tag{17}$$

and where $\delta_{\nu,\hat{N}}$ is a Kronecker $\delta$-operator symbol. $P(\nu)$ satisfies the expected normalization condition

$$\sum_{\nu=0}^{\infty} P(\nu) = 1. \tag{18}$$

It is easy to prove that the functions $P(\nu), E_p(\nu), N_p(\nu)$ are real.

With the particle number fixed, the chemical potential $\mu$ becomes a stability parameter. One chooses a value of $\mu$ that will generate a grand canonical ensemble average particle number close to the range of fixed particle numbers that one wishes to simulate. The accuracy of the evaluated numerical observables can be ascertained by the quality of the relation $N_p(\nu) - \nu \equiv 0$, which appears to be satisfied with an accuracy of $\approx 10^{-6}$ or better in a particle window of width a fraction of $N$, for systems with up to $N \approx 10^3$ particles. By changing $\mu$ and keeping $\beta$ constant one can map $E(N, \beta)$ in a large particle number $N$ interval.

In the case of interacting particles, after performing a Hubbard-Stratonovich transformation one obtains

$$\mathcal{Z}(\varphi) = \mathrm{Tr}\left[e^{-i\varphi(\hat{N}-N)} \int \mathcal{D}\sigma e^{-\tau(\hat{h}(\sigma)-\mu\hat{N})}\right], \tag{19a}$$
$$= \int \mathcal{D}\sigma P(\sigma) e^{i\varphi N} \det\left[\frac{1 + e^{-i\varphi}U}{1+U}\right], \tag{19b}$$
$$P(\sigma) = \frac{\det[1+U]}{Z}, \qquad \int \mathcal{D}\sigma P(\sigma) = 1, \tag{19c}$$

where we omit the $\sigma$ dependence of $U$ for clarity, and otherwise $U$ is the usual product of imaginary-time evolution operators

$$U = U_1 U_2 \ldots U_{N_\tau}. \tag{20}$$

The "observable" $e^{i\varphi N} \det\left[(1 + e^{-i\varphi}U)/(1+U)\right]$ has a Gaussian-like behavior as a function of $\varphi$. Similar expressions are obtained for other "observables" $\mathcal{E}(\varphi)$ and $\mathcal{N}(\varphi)$. After a QMC trajectory has been accepted, we evaluate $P(\nu)$, $E(\nu)$, and $N(\nu)$, and average over the Fourier-transformed "$\nu$-observables" rather than the original "$\varphi$-observables."

In a system with two (or more) types of particles at a finite temperature one can make separate particle projections for each type of fermion, by using two (or more) angles, e.g. $\varphi_\uparrow$ and $\varphi_\downarrow$ in the case of two flavors.

### 2. *Projecting particle number asymmetry in the case of two fermion flavors*

In the case of two flavors one can introduce the particle number asymmetry projection only. Let us consider a spin-1/2 fermion system

$$\hat{N}_+ = \hat{N}_\uparrow + \hat{N}_\downarrow, \tag{21a}$$
$$\hat{N}_- = \hat{N}_\uparrow - \hat{N}_\downarrow, \tag{21b}$$
$$\hat{N}_\sigma = \sum_{\mathbf{k}} \hat{\psi}^\dagger_\sigma(\mathbf{k})\hat{\psi}_\sigma(\mathbf{k}), \tag{21c}$$

where $\sigma = \uparrow, \downarrow$. We now introduce a new type of partition function and the related expectation values

$$\mathcal{W}(\theta) = \exp\left[-\beta(\hat{H} - \mu\hat{N}) - i\theta(\hat{N}_\uparrow - \hat{N}_\downarrow)\right], \tag{22a}$$
$$W(\theta) = \frac{1}{Z}\mathrm{Tr}\left[\mathcal{W}(\theta)\right] = \left\langle \exp\left[-i\theta(\hat{N}_\uparrow - \hat{N}_\downarrow)\right]\right\rangle, \tag{22b}$$
$$E(\theta) = \left\langle \hat{H} \exp\left[-i\theta(\hat{N}_\uparrow - \hat{N}_\downarrow)\right]\right\rangle, \tag{22c}$$
$$N_+(\theta) = \left\langle \hat{N}_+ \exp\left[-i\theta(\hat{N}_\uparrow - \hat{N}_\downarrow)\right]\right\rangle, \tag{22d}$$
$$N_-(\theta) = \left\langle \hat{N}_- \exp\left[-i\theta(\hat{N}_\uparrow - \hat{N}_\downarrow)\right]\right\rangle, \tag{22e}$$

The partition function $W(\theta)$ in Eq. (22b) is reminiscent of the partition function in studies that use an imaginary chemical potential $ih = i(\mu_\uparrow - \mu_\downarrow)/2$ as an asymmetry parameter [22–27]. Those studies, however, require analytic continuation to recover a real-valued asymmetry parameter, whereas this method requires no analytic continuation and, as we shall see, is without a sign problem.

The quantities in Eqs. (22b) to (22e) are functions of $\theta$ with period $2\pi$. Using them one can introduce a new type of grand canonical expectation with fixed polarization:

$$P(\eta) = \int_{-\pi}^{\pi} \frac{d\theta}{2\pi} \exp(i\eta\theta) W(\theta), \tag{23a}$$
$$E(\eta) = \frac{1}{P(\eta)} \int_{-\pi}^{\pi} \frac{d\theta}{2\pi} \exp(i\eta\theta) E(\theta), \tag{23b}$$
$$N_\pm(\eta) = \frac{1}{P(\eta)} \int_{-\pi}^{\pi} \frac{d\theta}{2\pi} \exp(i\eta\theta) N_\pm(\theta). \tag{23c}$$

$P(\eta)$, with $\eta$ an integer argument, is the probability to find an exact spin polarization $\eta = \langle \hat{N}_\uparrow - \hat{N}_\downarrow\rangle$, in the

grand canonical ensemble

$$P(\eta) = \frac{1}{Z}\,\mathrm{Tr}\left[\delta_{\eta,\hat{N}_\uparrow-\hat{N}_\downarrow}\exp\Big[-\beta(\hat{H}-\mu\hat{N})\Big]\right]. \quad (24)$$

where $\delta_{\eta,\hat{N}_\uparrow-\hat{N}_\downarrow}$ is a Kronecker $\delta$-operator symbol. $P(\eta)$ satisfies the expected normalization condition

$$\sum_{\eta=-\infty}^{\infty} P(\eta) = 1. \quad (25)$$

In AFQMC simulations, after a Hubbard-Stratonovich transformation, we have

$$W(\theta) = \int \mathcal{D}\sigma P[\sigma]F[\sigma,\theta], \quad (26a)$$

$$F[\sigma,\theta] \equiv \left|\det\left[\frac{1+e^{-i\theta}U}{1+U}\right]\right|^2, \quad (26b)$$

$$P[\sigma] \equiv \frac{\det^2[1+U]}{Z}, \qquad \int \mathcal{D}\sigma P(\sigma) = 1. \quad (26c)$$

Consequently, we have for the expectation values $N_\pm(\theta)$ the following forms

$$N_+(\theta) = \frac{1}{Z}\,\mathrm{Tr}\left[\hat{N}_+\mathcal{W}[\theta]\right] \quad (27a)$$

$$= 2\int \mathcal{D}\sigma P[\sigma]F[\sigma,\theta]\,\mathrm{Re}\left\{\mathrm{Tr}\,\frac{e^{-i\theta}U}{1+e^{-i\theta}U}\right\}, \quad (27b)$$

$$N_-(\theta) = \frac{1}{Z}\,\mathrm{Tr}\left[\hat{N}_-\mathcal{W}[\theta]\right] \quad (27c)$$

$$= 2\int \mathcal{D}\sigma P[\sigma]F[\sigma,\theta]\,\mathrm{Im}\left\{\mathrm{Tr}\,\frac{e^{-i\theta}U}{1+e^{-i\theta}U}\right\}, \quad (27d)$$

and similar relations for the other quantities $Z(\theta)$, $E(\theta)$, $N_\pm(\theta)$. As with the particle number projection, a good measure of the accuracy of the simulation is to compute the accuracy of the relation $N_-(\eta) - \eta \equiv 0$.

One benefit of constraining only the particle asymmetry as opposed to the total particle number is the positive definiteness of the terms in Eqs. (26a) to (26c), thereby avoiding the sign problem incurred when projecting total particle number.

#### 3. *Simultaneous projection of total particle number and particle number difference in the case of two fermion flavors*

One can combine the projection methods of Sections II B 1 and II B 2 to project on a specific combination of total particle number and particle difference (equivalent to constraining values for $N_\uparrow$ and $N_\downarrow$). We introduce a new statistical weight, partition function, and related expectation values

$$\mathcal{X}(\varphi,\theta) = \exp\Big[-\beta(\hat{H}-\mu\hat{N}) - i\varphi(\hat{N}_+ - N) - i\theta\hat{N}_-\Big], \quad (28a)$$

$$X(\varphi,\theta) = \frac{1}{Z}\,\mathrm{Tr}\left[\mathcal{X}(\varphi,\theta)\right]$$

$$= \Big\langle \exp\Big[-i\varphi(\hat{N}_+ - N) - i\theta\hat{N}_-\Big]\Big\rangle, \quad (28b)$$

$$E(\varphi,\theta) = \Big\langle \hat{H}\exp\Big[-i\varphi(\hat{N}_+ - N) - i\theta\hat{N}_-\Big]\Big\rangle, \quad (28c)$$

$$N_+(\varphi,\theta) = \Big\langle \hat{N}_+\exp\Big[-i\varphi(\hat{N}_+ - N) - i\theta\hat{N}_-\Big]\Big\rangle, \quad (28d)$$

$$N_-(\varphi,\theta) = \Big\langle \hat{N}_-\exp\Big[-i\varphi(\hat{N}_+ - N) - i\theta\hat{N}_-\Big]\Big\rangle. \quad (28e)$$

As before, we introduced the additional phase factor of $\exp(i\varphi N)$ for numerical stability. Without this phase factor, the "observables" are periodic functions of $\varphi$, with a period of $2\pi$ and they satisfy similar relations to those in Eq. (15c). One then introduces the particle projected expectation values

$$P(\nu,\eta) = \int_{-\pi}^{\pi}\frac{d\varphi}{2\pi}\int_{-\pi}^{\pi}\frac{d\theta}{2\pi}e^{i\nu\varphi}e^{i\eta\theta}X(\varphi,\theta), \quad (29a)$$

$$E(\nu,\eta) = \frac{1}{P(\nu,\eta)}\int_{-\pi}^{\pi}\frac{d\varphi}{2\pi}\int_{-\pi}^{\pi}\frac{d\theta}{2\pi}e^{i\nu\varphi}e^{i\eta\theta}E(\varphi,\theta), \quad (29b)$$

$$N_\pm(\nu,\eta) = \frac{1}{P(\nu,\eta)}\int_{-\pi}^{\pi}\frac{d\varphi}{2\pi}\int_{-\pi}^{\pi}\frac{d\theta}{2\pi}e^{i\nu\varphi}e^{i\eta\theta}N_\pm(\varphi,\theta). \quad (29c)$$

$P(\nu,\eta)$ is the probability to find states that satisfy both $\langle\hat{N}_+\rangle - N = \nu$ and $\langle\hat{N}_-\rangle = \eta$ in the grand canonical ensemble and it satisfies the normalization condition

$$\sum_{\nu=-\infty}^{\infty}\sum_{\eta=-\infty}^{\infty} P(\nu,\eta) = 1. \quad (30)$$

In our AFQMC simulations, after a Hubbard-Stratonovich transformation, we will calculate

$$X(\varphi,\theta) = \int \mathcal{D}\sigma P[\sigma]F[\sigma,\varphi,\theta], \quad (31a)$$

$$F[\sigma,\varphi,\theta] \equiv e^{i\varphi N}\frac{1}{\det^2[1+U]}\det\left[1+e^{-i(\varphi+\theta)}U\right] \times \det\left[1+e^{-i(\varphi-\theta)}U\right], \quad (31b)$$

$$P[\sigma] \equiv \frac{\det^2[1+U]}{Z}, \qquad \int \mathcal{D}\sigma P(\sigma) = 1. \quad (31c)$$

Section VII details practical considerations for calculating these observables stably and efficiently.

## III. TAN CONTACT, $C$

In addition to thermodynamic probes measured in the main text, we also calculate the Tan contact $C$, which

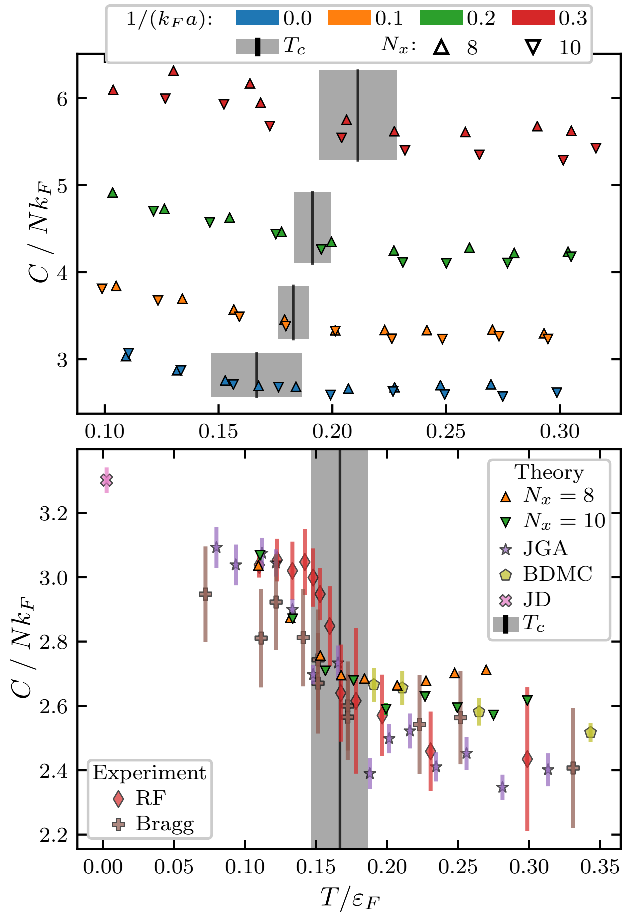


FIG. 2. AFQMC results for the Tan contact derived from Eq. (35) for $0.0 \leq 1/(k_Fa) \leq 0.3$. (upper panel) The Tan contact decreases monotonically as temperature increases and increases as $1/(k_Fa)$ increases. The shaded boxes indicate the critical temperature with error bounds at the specified scattering length. Error bars for the contact estimates are within the marker size. (lower panel) We compare to other studies: experimental results based on radio frequency spectral response of Mukherjee *et al.* [28] (labeled as RF); an experimental study using focused beam Bragg spectroscopy from Carcy *et al.* [29] (labeled as Bragg); a previous QMC study at zero temperature from Drut [30] (JD); a bold diagrammatic Monte Carlo result from Rossi *et al.* [31] (BDMC); and a previous constrained ensemble AFQMC study from Jensen *et al.* [32] (JGA).

parameterizes all short range correlations in the system. It is a central property of systems of fermions with large scattering lengths, with relations concerning the tail of the momentum distribution [33],

$$C \equiv \lim_{k\to\infty} k^4 n_\sigma(k), \tag{32}$$

where $n_\sigma(k)$ is the momentum distribution for particles with spin $\sigma$ and momentum $k$; the thermodynamic derivative of the free energy with respect to the scattering length [34]

$$\frac{\partial F}{\partial a^{-1}} = -\frac{\hbar^2}{4\pi m}C; \tag{33}$$

and the pressure and energy density of a homogeneous system [35]:

$$\mathcal{P} = \frac{2}{3}\mathcal{E} + \frac{\hbar^2}{12\pi m a}C. \tag{34}$$

See Braaten [36] for a review of the Tan contact.

Following Jensen *et al.* [32], we calculate $C$ in the lattice formulation as

$$C = \frac{m^2 g \left\langle \hat{V} \right\rangle}{\hbar^4}, \tag{35}$$

where $\langle \hat{V} \rangle$ is the expectation value of the potential energy operator. In Fig. 2, we show our results for the Tan contact at multiple scattering lengths, with shaded boxes indicating the critical temperature, with error bounds. The Tan contact increases as we increase $1/(k_Fa)$ and decreases with decreasing temperature.

To our knowledge, our results for $0.1 \leq 1/(k_Fa) \leq 0.3$ are the first published finite-temperature estimates of the Tan contact away from unitarity, thus preventing comparison to previous results. However, at unitarity we compare our results to previous studies in the lower panel of Fig. 2.

Positing a link between contact and pairing, Pieri *et al.* [37] have argued that the Tan contact measures local pairing as $C = (m\Delta_\infty)^2$. This parameter was first introduced by Pieri *et al.* [37] and later generalized by Rossi *et al.* [31]. However, the exact relationship between $\Delta_\infty$ and the superconducting order parameter $\Delta$ remains elusive. In Fig. 3, we show our normalized results for $\Delta_\infty$

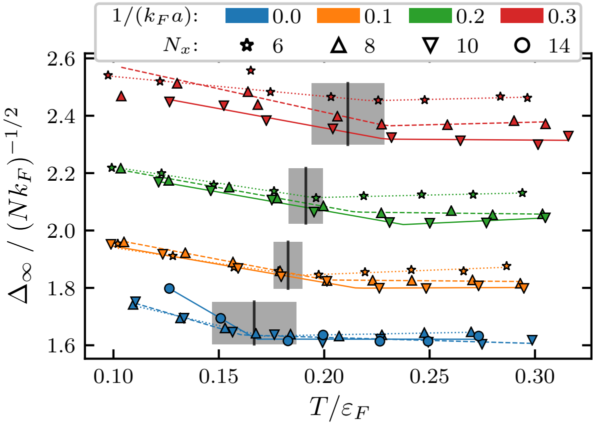


FIG. 3. AFQMC results for the contact-derived pairing parameter $\Delta_\infty$ using Eq. (36). $\Delta_\infty$ displays clearly different low and high temperature structure. We fit a piecewise linear function and define the "switching temperature" as a new characteristic temperature, $T_\infty$. We record $T_\infty$ in Table I.

derived from the Tan contact using

$$\frac{\Delta_\infty}{\sqrt{Nk_F}} \equiv \frac{1}{m}\sqrt{\frac{C}{Nk_F}}. \tag{36}$$

We find no obvious relationship between $\Delta_\infty$ and the even-odd staggering pairing gap. However, $\Delta_\infty$ has distinct low- and high-temperature behaviors, with an almost linear decrease from a maximum at the lowest temperature to a "switching temperature" where $\Delta_\infty$ levels off or, in the case of small lattices, increases gradually. We fit these curves to a piecewise linear fit and record the "switching" temperature as a new characteristic temperature, $T_\infty$, in Table I.

TABLE I. Characteristic temperatures in the BCS–BEC crossover. $T_c$ is the superfluid critical temperature. $T_s$ is the temperature at which the spin susceptibility peaks. $T^*$ is the temperature at which the pairing gap disappears. $T_\infty$ is the temperature that separates the low and high temperature behaviors of the Tan contact-derived pairing parameter $\Delta_\infty$. $T_c$ estimates are compatible with previous estimates by Burovski *et al.* [38] and Bulgac *et al.* [1]. Estimates for $T^*$ are compatible with previous results by Magierski *et al.* [39].

| $1/(k_F a)$ | $T_c/\varepsilon_F$ | $T^*/\varepsilon_F$ | $T_s/\varepsilon_F$ | $T_\infty/\varepsilon_F$ |
|---|---|---|---|---|
| 0.0 | 0.16(2) | 0.21(3) | > 0.24(1) | 0.166(5) |
| 0.1 | 0.183(6) | 0.22(2) | > 0.28(1) | 0.20(1) |
| 0.2 | 0.191(8) | 0.26(3) | > 0.30 | 0.22(2) |
| 0.3 | 0.21(2) | 0.28(2) | > 0.30 | 0.23(1) |

However, we caution that our identification of $T_\infty$ is a speculative characteristic temperature. We therefore refrain from making inferences about the pseudogap using measurements of $\Delta_\infty$ or $T_\infty$ until the relationship between $\Delta_\infty$ and the pairing gap $\Delta$ is clarified. This issue warrants further study.

## IV. FINITE SIZE SCALING OF THE CONDENSATE FRACTION

Near the critical temperature, the condensate fraction $\alpha$ that serves as the order parameter for off-diagonal long range order (ODLRO), has a well-established scaling behavior given by the renormalization group theory [40],

$$R(T,L) = \alpha(T)L^{1+\eta} = f(x)\left(1 + cL^{-\omega} + \ldots\right), \tag{37}$$

where $L$ is the lattice size, $\eta = 0.038$ is a universal critical exponent and $f(x)$ is a universal analytic function of $x \equiv (N_x/\xi_{\text{corr}})^{1/\nu}$, with $\xi_{\text{corr}}$ being the correlation length and $\nu$ being another universal critical exponent, $\nu = 0.671$. In Eq. (37), $c$ is an unknown, non-universal constant, and $\omega \approx 0.8$ is the critical exponent of the leading irrelevant field. The $T$-dependence in the right-hand-side of Eq. (37) is hidden in the correlation length, which diverges near $T_c$ as

$$\xi_{\text{corr}} \propto |1 - T/T_c|^{-\nu}, \tag{38}$$

sending $x$ to 0.

For each scattering length, we compute $R(T,L)$ for multiple lattice sizes and multiple temperatures. We then find "crossing temperatures" $T_{ij}$ at which $R(L_i,T_{ij}) = R(L_j,T_{ij})$. In the left column of Fig. 4, we show $R(T,L)$ for each scattering length, indicating the crossing temperatures $T_{ij}$ with multicolored markers.

One then expands the universal function as $f(x) = f(0) + f'(0)L^{1/\nu}b|1 - T/T_c|$, where $b$ is a proportionality constant, yielding

$$|T_c - T_{ij}| = \kappa g\left(L_i, L_j\right) \tag{39a}$$

where

$$\kappa = \frac{cT_c f(0)}{bf'(0)} \tag{39b}$$

and

$$g\left(L_i,L_j\right) = L_j^{-(\omega+1/\nu)}\left[\frac{\left(\frac{L_j}{L_i}\right)^{\omega} - 1}{1 - \left(\frac{L_i}{L_j}\right)^{1/\nu}}\right]. \tag{39c}$$

In the thermodynamic limit, $L \to \infty$ and $g(L_i,L_j) \to 0$, we recover the true critical temperature. We therefore extrapolate the crossing temperatures $T_{ij}$ to the thermodynamic limit, taking care to propagate the errors in $\alpha$ to the crossing temperatures $T_{ij}$ and then to the extrapolated $T_c$. In the right column of Fig. 4, we show the crossing temperatures $T_{ij}$ and extrapolation to the thermodynamic limit. The errors in our estimates of $T_c$ are therefore affected by the errors in $\alpha$ and also by the residuals of the linear fit in Fig. 4.

## V. EXTRACTING $\Delta$ AND $\xi(T)$ FROM EVEN-ODD ENERGY STAGGERING

We used two different methods to estimate $\Delta_E$: the five-point difference formula

$$\Delta_E^{(5)} = \frac{(-1)^N}{8}\sum_{s=\pm1}\Big[4E(N+s) - E(N+2s) - 3E(N)\Big], \tag{40}$$

and the equation of state (EOS) fit

$$E/E_{FG}(\xi,\Delta_E^{(f)}) = \xi + |N_-|\frac{\Delta_E^{(f)}}{E_{FG}}. \tag{41}$$

These pairing gap estimates require accurate computation of the ground state energy at fixed particle numbers and reduced temperature $T/\varepsilon_F$. For each grand canonical simulation, we projected fixed, integer-valued particle numbers in the range $\langle N\rangle_{GCE} - 4 \le N \le \langle N\rangle_{GCE} + 4$, where $\langle N\rangle_{GCE}$ is the average particle number in the grand canonical ensemble. This range resulted in nine projected particle numbers and was chosen to satisfy

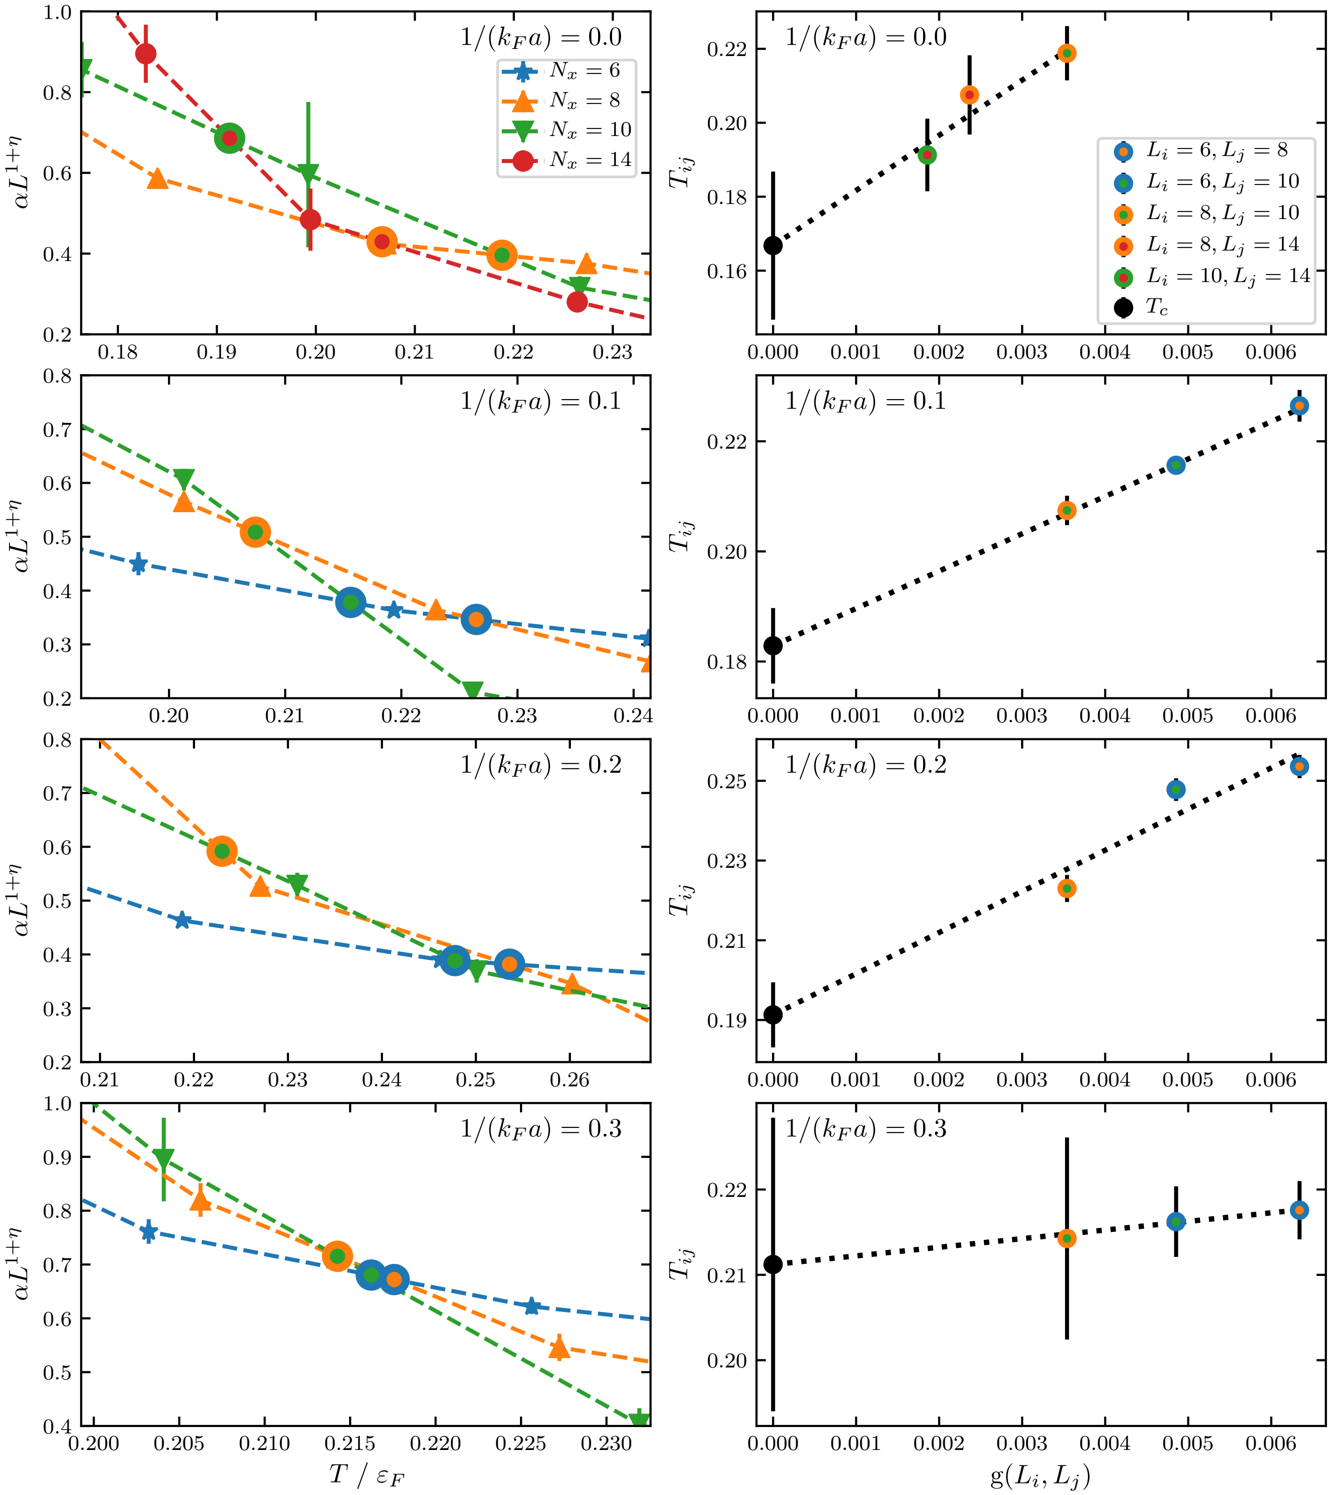


FIG. 4. (left column) The scaled order parameter $R(T, L)$ from Eq. (37) for multiple lattice sizes and scattering lengths. The crossing temperatures where $R(T, L)$ for two different lattices intersect are indicated by the multicolored markers (see legend in right panel). (right column) The crossing temperatures $T_{ij}$ derived from the intersections in the left column are extrapolated to the infinite limit. Black circles at $g(L_i, L_j) = 0$ represent our estimates of $T_c$. Because we used larger lattices at unitarity, the $T_{ij}$ values are closer to the $y$-axis than at other coupling strengths.

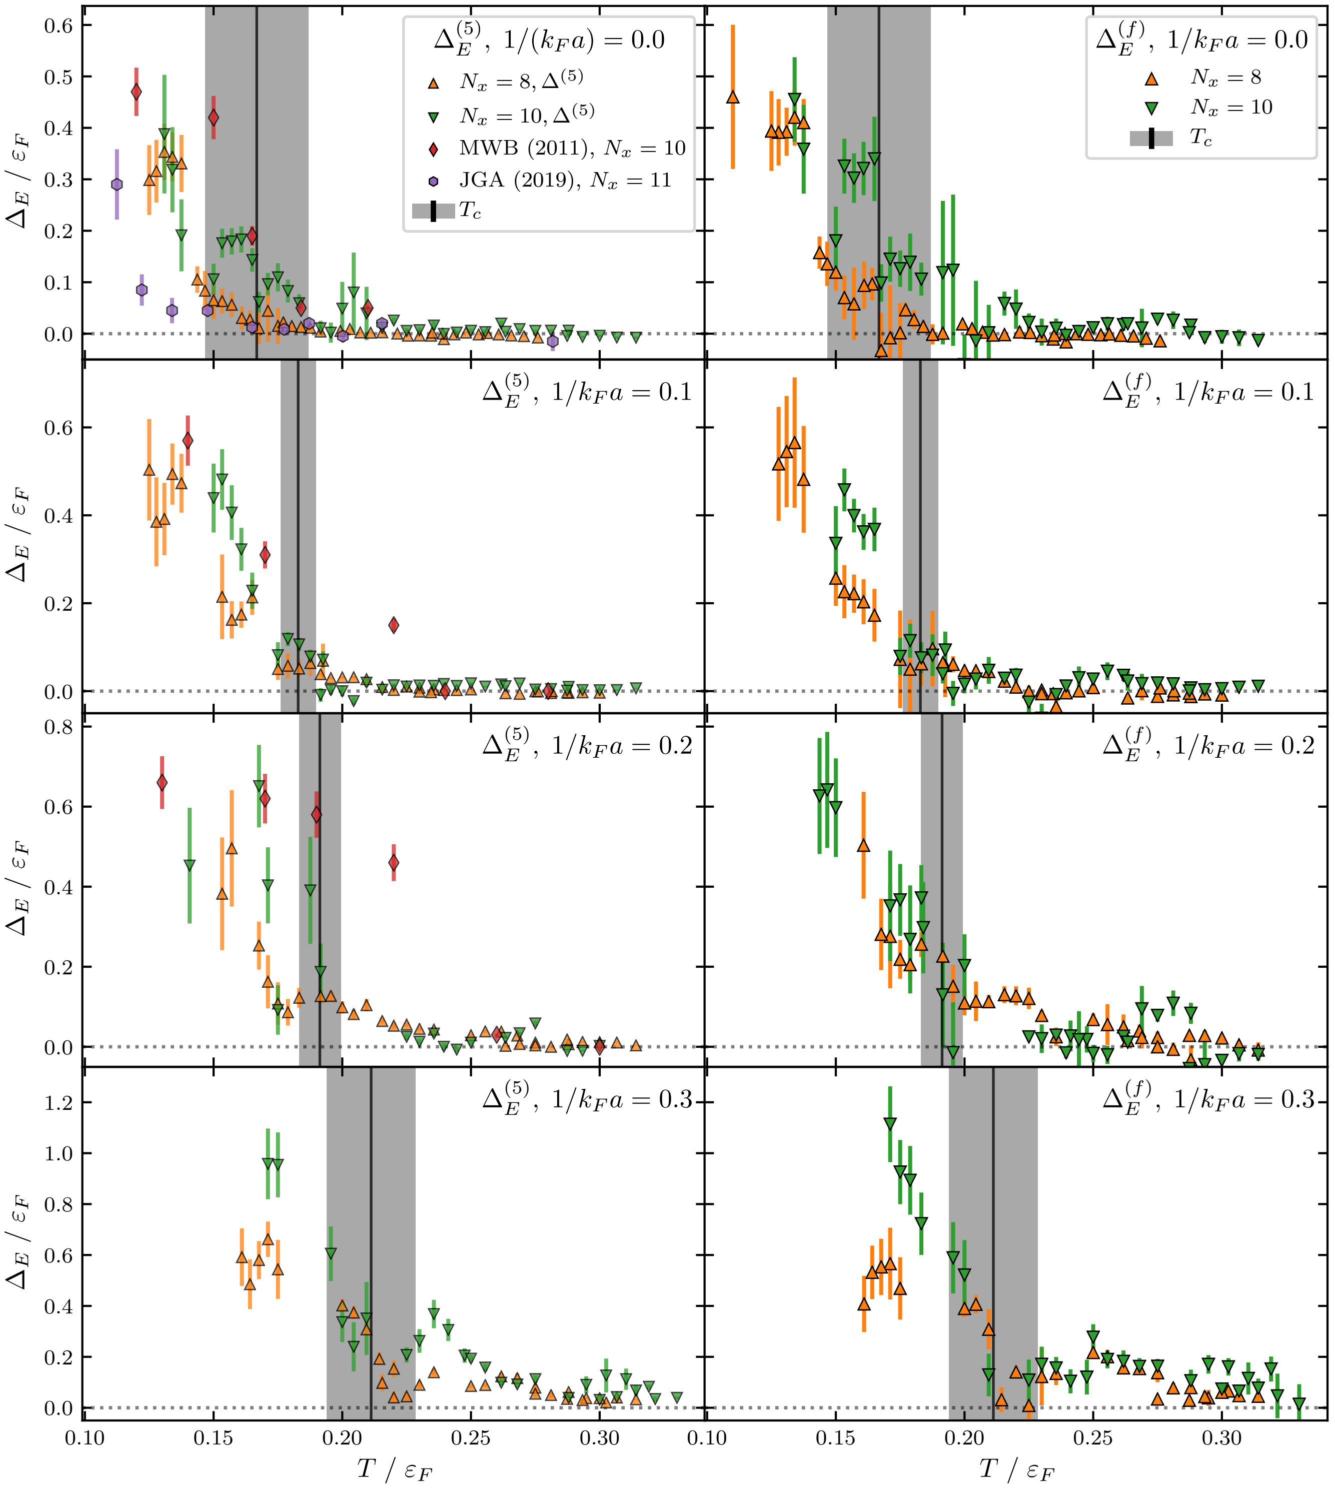


FIG. 5. Left: AFQMC results for the pairing gap $\Delta_E$ extracted from even-odd energy staggering using the five-point difference formula in Eq. (40). At unitarity, we compare our results to a previous study extracting the gap from the spectral weight function, labeled as MWB [39] and one extracting the gap from the three-point even-odd energy staggering, labeled as JGA [20]. At $0.1 \le 1/(k_F a) \le 0.3$, We compare our results to the MWB values when they are available for the scattering length. However, one should be careful comparing the MWB values since they measure the spectral gap, which is *a priori* different from the even-odd energy staggering. Right: AFQMC results for the pairing gap extracted from even-odd energy staggering using Eq. (41). The results for $\Delta_E^{(f)}$ are in rough agreement with those for $\Delta_E^{(5)}$ derived from the five-point difference formula.

$|N-\nu| < 10^{-6}$, where $N$ is the measured particle number and $\nu$ is the target particle number. The corresponding energies for these systems were all computed at the same absolute temperature $T$ but had slightly different reduced temperatures $T/\varepsilon_F$ due to changes in particle number, thereby spreading the measurements of the pairing gap spread across a range of reduced temperatures centered on the reduced temperature of the grand canonical ensemble. Thus a single GCE simulation constrained to nine different particle numbers, would produce five estimates of $\Delta_E^{(5)}$ at slightly different reduced temperatures. In Section IX, we discuss these details and further steps involved in correctly calculating these energies.

As the temperature decreases, the grand canonical ensemble becomes more tightly distributed around $\langle\hat{N}\rangle_{GCE}$ and the particle number projection requires sampling farther out into the tails of the GCE, increasing the sampling error. For this reason, errors in the pairing gap estimates become large for low temperatures. Luckily, we are interested in the regime $T_c \leq T \leq T^*$, where the errors are more manageable.

For the five-point difference formula, each fit takes energies from five different particle numbers and $\eta \in \{0,1\}$. An example stagger plot is shown in Fig. 6 for $1/(k_F a) = 0$, $N_x = 8$, and $T/\varepsilon_F = 0.15$, to aid in understanding exactly which points are included in each fit. Each five-point estimate has a different central particle number and therefore a different reduced temperature $\widetilde{T} \equiv T/\varepsilon_F$ (further explained in Section IX C). Each simulation of the GCE therefore generates five different estimates of $\Delta_E^{(5)}$ at five different reduced temperatures centered around the reduced temperature of the GCE. In the left column of Fig. 5, we show our results for $\Delta_E^{(5)}$ and compare to previous studies when available.

In addition to estimating $\Delta_E$ using the five-point difference, we also estimate $\Delta_E$ by fitting the energies to the equation of state in Eq. (41) where $\xi$ is a temperature-dependent generalization of the Bertsch parameter (i.e. a dimensionless universal parameter). We show our results for $\Delta_E^{(f)}$ in the right column of Fig. 5 and find broad agreement between $\Delta_E^{(f)}$ and $\Delta_E^{(5)}$.

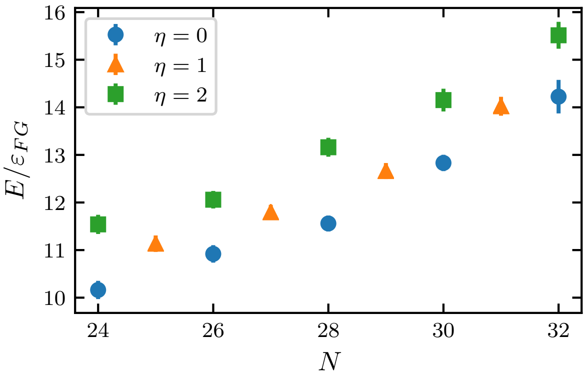


FIG. 6. An example stagger plot for $1/(k_F a) = 0$, $N_x = 8$, and $T/\varepsilon_F = 0.125$. The energy is normalized to the energy per particle of the free Fermi gas, as in Carlson *et al.* [41] and Chang *et al.* [42]. We show points for $\eta \in \{0,1,2\}$. With nine different particle number values, this stagger plot would yield five estimates of $\Delta_E^{(5)}$ and $\Delta_E^{(f)}$ each.

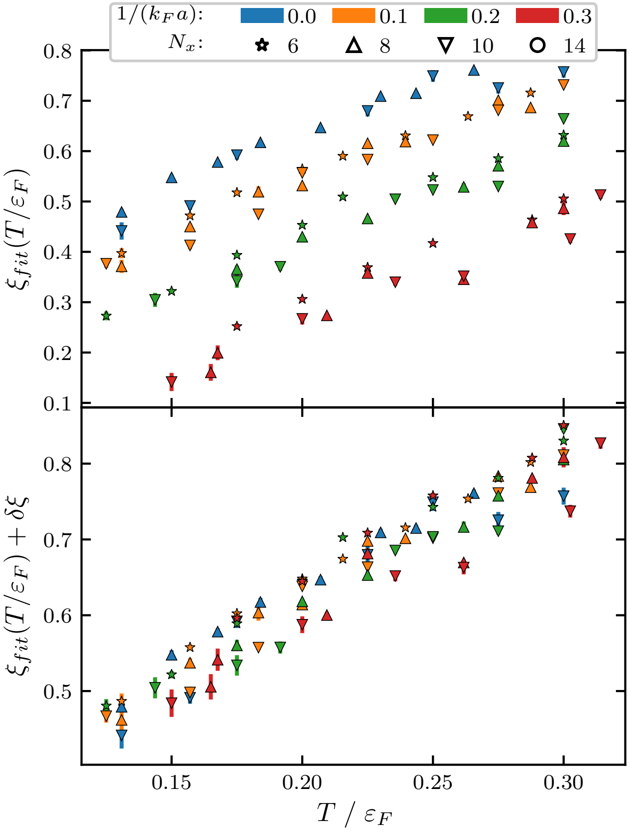


FIG. 7. AFQMC results for the temperature dependent Bertsch parameter $\xi(T)$ obtained by fitting energies to Eq. (41). In the upper panel, we show our results for $\xi(T)$ at $0.0 \leq 1/(k_F a) \leq 0.3$. In the lower panel, we show $\xi(T) + \delta\xi$, where $\delta\xi$ is the energy shift obtained from the Tan contact defined in Eq. (42b).

To estimate $T^*$ we fit both $\Delta_E^{(5)}$ and $\Delta_E^{(f)}$ using a univariate cubic spline. This allows us to easily compute the roots and derivatives of the interpolant. Denoting the interpolant function by $\widehat{\Delta}$, and the first root of some function $f$ as $\omega[f]$, we then define our estimate for $T^*$ as the minimum of the first root of the interpolant and the first plateau (zero derivative) of the interpolant: $T^* = \min(\omega[\widehat{\Delta}], \omega[\partial_T \widehat{\Delta}])$. Our estimates of $T^*$ are listed in Table I.

The fitting function in Eq. (41) also allows us to estimate the temperature-dependent Bertsch parameter $\xi(T)$. We show our estimates for $\xi(T)$ in Fig. 7. Because these results are obtained from fitting energies calculated in the constrained ensemble, we do not expect high pre-

cision results like those in [4]. However, the estimates of $\xi$ do serve as a consistency check on the constrained ensemble. We can also check the consistency of the Tan contact using Eq. (33):

$$\frac{\partial E}{\partial 1/(k_F a)} = \frac{\hbar^2 k_F C}{4\pi m}, \tag{42a}$$

$$\Rightarrow \frac{\partial \xi(T)}{\partial (k_F a)^{-1}} = \frac{\partial (E\,/\,E_{FFG})}{\partial (k_F a)^{-1}} = -\frac{5}{6\pi}\frac{C}{Nk_F}. \tag{42b}$$

In the lower panel of Fig. 7, we use Eq. (42b) to shift all estimates of $\xi(T)$ for $0.1 \le 1/(k_F a) \le 0.3$ up to unitarity. This application of the Tan contact derived from the GCE to an equation of state derived from the doubly constrained (both $N_+$ and $N_-$) ensemble serves as a consistency check on our Tan contact results and the constrained ensemble method.

## VI. GAUSSIAN PROCESS REGRESSION OF $\xi$ AND $\Delta$

The temperature "smearing" effect described in Section V, and in more detail in Section IX C, combined with the multiple methods for estimating $\Delta_E$ lead to a profusion of observations that make it difficult to visualize and compare our results to others. The same surplus of observations occurs for $\xi$, with multiple estimates coming from Eq. (41) and from measurements of $E/E_{FFG}$ in the GCE.

To resolve this, we use a Gaussian process (GP) regressor to interpolate our data. A similar approach is used in nuclear theory, where an abundance of competing nuclear mass models make different predictions for nuclear separation energies and one wishes to extrapolate far from the valley of stability [43], with one key difference being that we use GP regression to interpolate rather than extrapolate. GPs have also been used for parameter estimation in chiral effective field theories [44].

GP regression is a non-parametric, Bayesian approach to regression, in which we treat our results as a training set for a new statistical model for each scattering length. For $\Delta_E$, the training set includes all measurements of $\Delta_E^{(5)}$ and $\Delta_E^{(f)}$ for all lattice sizes $N_x \ge 8$. For $\xi$, the training set includes all measurements of $\xi$ from Eq. (41) and of $E/E_{FFG}$ from the GCE, for lattice sizes $N_x \ge 8$. Because we use GPs for interpolation and clarity in plotting, and not for estimation of $T^*$, we do not use cross-validation or split our data into training, testing, and validation sets, which is de rigueur when building a model to predict new results [45].

We briefly introduce the key concepts of GP regression and refer the reader to Williams and Rasmussen [46] for a more thorough, pedagogical introduction. Let $\mathbf{y}$ be the target vector of measurements we wish to interpolate (either $\Delta_E$ or $\xi$) and $\mathbf{x}$ be the input vector of temperatures $T/\varepsilon_F$. We wish to find a real process $f(\mathbf{x},\theta)$ that will model and predict new target output given arbitrary inputs,

$$\mathbf{y} = f(\mathbf{x},\theta) + \epsilon, \tag{43}$$

where $\theta$ encapsulates the parameters of our statistical model and $\epsilon$ represents identically distributed Gaussian noise, with zero mean and variance $\sigma^2$, which differentiates the observed values from the function values. Following the "function-space view" [46], one can define the mean $m(\mathbf{x})$ and covariance $k(\mathbf{x},\mathbf{x}')$ of $f(\mathbf{x})$ as

$$\mu(\mathbf{x}) = \mathbb{E}\left[f(\mathbf{x}))\right], \tag{44}$$

$$k(\mathbf{x},\mathbf{x}') = \mathbb{E}\left[(f(\mathbf{x}) - \mu(\mathbf{x}))(f(\mathbf{x}') - \mu(\mathbf{x}'))\right], \tag{45}$$

and approximate $f(\mathbf{x})$ by a Gaussian process

$$f(\mathbf{x}) \approx \mathcal{GP}\left(\mu(\mathbf{x}), k_\theta(\mathbf{x},\mathbf{x}')\right), \tag{46}$$

which is completely specified by its mean and covariance functions. We take the covariance function to be the weighted sum of a $\nu = 3/2$ Matérn kernel and a white noise kernel

$$k(d_{ij}) = \underbrace{\eta^2\left(1 + \frac{\sqrt{3}d_{ij}}{\rho}\right)e^{\left(-\frac{\sqrt{3}d_{ij}}{\rho}\right)}}_{\text{Matérn}} + \underbrace{\delta_{ij}\varepsilon}_{\text{white noise}}, \tag{47}$$

where $d_{ij} \equiv |x_i - x_j|$ and $\delta_{ij}$ is the Kronecker delta. The Matérn kernel is a generalization of the popular radial-basis function (RBF or "squared exponential") kernel, and is appropriate for learning functions that are at least once differentiable, in contrast to the assumption of infinite differentiability with the RBF kernel [46, 47]. Thus, our statistical model has four parameters $\theta := (\mu, \eta, \rho, \varepsilon)$: the mean $\mu$, the correlation strength $\eta$, the Matérn coherence length $\rho$, and the noise level $\varepsilon$.

GP regression estimates the parameters $\theta$ by specifying a prior distribution $p(\theta)$ and relocating those probabilities based on Bayes rule

$$p(\theta|\mathbf{y},\mathbf{x}) = \frac{p(\mathbf{y}|\mathbf{x},\theta)\,p(\theta)}{p(\mathbf{y}|\mathbf{x})}, \tag{48}$$

where the marginal likelihood $p(\mathbf{y}|\mathbf{x})$ is given by

$$p(\mathbf{y}|\mathbf{x}) = \int p(\mathbf{y}|\mathbf{x},\theta)\,p(\theta)d\theta. \tag{49}$$

For each observable, $\xi$ and $\Delta$, and at each scattering length, we perform this parameter optimization using *scikit-learn*'s `GaussianProcessRegressor` object [48], with the L-BGFS-B minimization algorithm from `scipy.optimize.minimize` [49].

In Table II, we present the predictions of our GP models at regularly spaced temperature values, omitting temperatures that fall outside of the range of input data at each scattering length. We used our GP models to plot and compare $\xi$ and $\Delta_E$ in the main text, however the spline fits described in Section V, from which we computed $T^*$, were computed on the input $\Delta_E$ estimates rather than the GP predictions. The fact that the computed $T^*$ values also describe the disappearance of the GP predictions serves as a preliminary consistency check of our GP models.

TABLE II. Predictions of the Gaussian process regressors for $\xi$ and $\Delta$, described in Section VI. $\sigma_{\bar{x}}$ denotes the standard error of the mean of $x$. We omit values that extrapolate outside of our data range.

| $T/\varepsilon_F$ | $1/(k_Fa)=0.0$ | | | | $1/(k_Fa)=0.1$ | | | | $1/(k_Fa)=0.2$ | | | | $1/(k_Fa)=0.3$ | | | |
|---|---|---|---|---|---|---|---|---|---|---|---|---|---|---|---|---|
| | $\xi$ | $\sigma_{\bar{\xi}}$ | $\Delta$ | $\sigma_{\bar{\Delta}}$ | $\xi$ | $\sigma_{\bar{\xi}}$ | $\Delta$ | $\sigma_{\bar{\Delta}}$ | $\xi$ | $\sigma_{\bar{\xi}}$ | $\Delta$ | $\sigma_{\bar{\Delta}}$ | $\xi$ | $\sigma_{\bar{\xi}}$ | $\Delta$ | $\sigma_{\bar{\Delta}}$ |
| 0.10 | 0.44 | 0.03 | – | – | 0.32 | 0.02 | – | – | 0.22 | 0.03 | – | – | 0.06 | 0.04 | – | – |
| 0.11 | 0.46 | 0.02 | 0.28 | 0.06 | 0.34 | 0.02 | – | – | 0.23 | 0.03 | – | – | 0.07 | 0.03 | – | – |
| 0.12 | 0.47 | 0.02 | 0.26 | 0.05 | 0.36 | 0.01 | 0.41 | 0.08 | 0.25 | 0.02 | – | – | 0.08 | 0.03 | – | – |
| 0.13 | 0.49 | 0.01 | 0.23 | 0.04 | 0.37 | 0.01 | 0.38 | 0.06 | 0.26 | 0.02 | – | – | 0.10 | 0.02 | – | – |
| 0.14 | 0.50 | 0.01 | 0.20 | 0.03 | 0.39 | 0.01 | 0.34 | 0.05 | 0.28 | 0.02 | 0.34 | 0.07 | 0.12 | 0.02 | – | – |
| 0.15 | 0.52 | 0.01 | 0.16 | 0.03 | 0.42 | 0.01 | 0.29 | 0.04 | 0.30 | 0.01 | 0.32 | 0.06 | 0.13 | 0.02 | – | – |
| 0.16 | 0.55 | 0.01 | 0.12 | 0.02 | 0.44 | 0.01 | 0.23 | 0.03 | 0.32 | 0.01 | 0.29 | 0.04 | 0.15 | 0.02 | 0.60 | 0.09 |
| 0.17 | 0.57 | 0.01 | 0.08 | 0.02 | 0.46 | 0.01 | 0.17 | 0.03 | 0.34 | 0.01 | 0.25 | 0.04 | 0.17 | 0.01 | 0.59 | 0.07 |
| 0.18 | 0.59 | 0.01 | 0.05 | 0.02 | 0.49 | 0.01 | 0.11 | 0.02 | 0.36 | 0.01 | 0.21 | 0.03 | 0.19 | 0.01 | 0.55 | 0.07 |
| 0.19 | 0.61 | 0.01 | 0.03 | 0.02 | 0.51 | 0.01 | 0.07 | 0.02 | 0.38 | 0.01 | 0.17 | 0.02 | 0.22 | 0.01 | 0.47 | 0.06 |
| 0.20 | 0.63 | 0.01 | 0.01 | 0.01 | 0.53 | 0.01 | 0.04 | 0.01 | 0.41 | 0.01 | 0.13 | 0.02 | 0.24 | 0.01 | 0.37 | 0.05 |
| 0.21 | 0.65 | 0.01 | 0.00 | 0.01 | 0.56 | 0.01 | 0.02 | 0.01 | 0.43 | 0.01 | 0.10 | 0.02 | 0.26 | 0.01 | 0.26 | 0.04 |
| 0.22 | 0.68 | 0.01 | 0.00 | 0.01 | 0.58 | 0.01 | 0.01 | 0.01 | 0.45 | 0.01 | 0.07 | 0.02 | 0.29 | 0.01 | 0.18 | 0.04 |
| 0.23 | 0.69 | 0.01 | 0.00 | 0.01 | 0.60 | 0.01 | 0.00 | 0.01 | 0.47 | 0.01 | 0.04 | 0.02 | 0.31 | 0.01 | 0.14 | 0.04 |
| 0.24 | 0.71 | 0.01 | 0.00 | 0.01 | 0.62 | 0.01 | 0.00 | 0.01 | 0.49 | 0.01 | 0.03 | 0.01 | 0.33 | 0.01 | 0.14 | 0.04 |
| 0.25 | 0.73 | 0.01 | 0.00 | 0.01 | 0.64 | 0.01 | 0.00 | 0.01 | 0.51 | 0.01 | 0.02 | 0.01 | 0.35 | 0.01 | 0.14 | 0.03 |
| 0.26 | 0.74 | 0.01 | 0.00 | 0.01 | 0.65 | 0.01 | 0.00 | 0.01 | 0.53 | 0.01 | 0.02 | 0.01 | 0.37 | 0.01 | 0.13 | 0.03 |
| 0.27 | 0.75 | 0.01 | 0.00 | 0.01 | 0.67 | 0.01 | 0.00 | 0.01 | 0.55 | 0.01 | 0.02 | 0.01 | 0.40 | 0.01 | 0.10 | 0.03 |
| 0.28 | 0.76 | 0.02 | 0.00 | 0.01 | 0.69 | 0.01 | 0.00 | 0.01 | 0.57 | 0.01 | 0.01 | 0.01 | 0.42 | 0.01 | 0.07 | 0.03 |
| 0.29 | 0.77 | 0.02 | 0.00 | 0.01 | 0.71 | 0.01 | 0.00 | 0.01 | 0.59 | 0.01 | 0.01 | 0.01 | 0.45 | 0.01 | 0.05 | 0.02 |
| 0.30 | 0.77 | 0.03 | 0.00 | 0.02 | 0.72 | 0.01 | 0.00 | 0.01 | 0.61 | 0.01 | 0.01 | 0.01 | 0.47 | 0.01 | 0.05 | 0.02 |

## VII. CALCULATING CONSTRAINED ENSEMBLE OBSERVABLES IN AFQMC

Here we outline the MCMC formalism to compute the observables $X(\varphi,\theta), E(\varphi,\theta), N_\pm(\varphi,\theta)$. In our notation, $U$ is the single particle basis representation of the usual product of imaginary-time evolution operators $U = U_1U_2\ldots U_{N_\tau}$. For the unconstrained grand canonical ensemble, we have $U_\uparrow = U_\downarrow = U$. Thus, when we explicitly include arrow subscripts, it is implied that we are calculating projected observables in the constrained ensemble. And when we omit the arrow subscripts, we are referencing a value calculated in the unconstrained grand canonical ensemble. For simultaneous projection of the total particle number and the particle difference between two flavors, we define $U_{\uparrow,\downarrow} = e^{-i(\varphi\pm\theta)}U$.

### A. Calculating occupation matrices

In the unconstrained grand canonical simulation, the imaginary time evolution operator is computed as a QDR decomposition

$$U = QDR, \tag{50}$$

$$1+U = Q\left[Q^\dagger R^{-1} + D\right]R = Q\widetilde{Q}\widetilde{D}\widetilde{R}R, \tag{51}$$

$$\begin{aligned} n &= \frac{U}{1+U} = 1 - \frac{1}{1+U} \\ &= 1 - R^{-1}\widetilde{R}^{-1}\widetilde{D}^{-1}\widetilde{Q}^\dagger Q^\dagger, \end{aligned} \tag{52}$$

where $Q$ and $\widetilde{Q}$ are unitary matrices, $D$ and $\widetilde{D}$ are diagonal matrices and $R$ and $\widetilde{R}$ are upper unit-triangular matrices.

To compute $U_\sigma$, one might naively expect to update the QDR decomposition at the end of the imaginary time evolution

$$U_\sigma = e^{-i\alpha_\sigma}QDR, \tag{53}$$

$$\begin{aligned} 1+U_\sigma &= Q\left[Q^\dagger R^{-1} + e^{-i\alpha_\sigma}D\right]R \\ &= Q\widetilde{Q}_\sigma\widetilde{D}_\sigma\widetilde{R}_\sigma R, \end{aligned} \tag{54}$$

$$n_\sigma = 1 - \frac{1}{1+U_\sigma} = 1 - R^{-1}\widetilde{R}_\sigma^{-1}\widetilde{D}_\sigma^{-1}\widetilde{Q}_\sigma^\dagger Q^\dagger, \tag{55}$$

where $\sigma \in \{\uparrow,\downarrow\}$ (not to be confused with the auxiliary field) and $\alpha_\sigma = (\varphi\pm\theta)$. However, we can avoid the cost of these extra QDR decompositions by writing the occupation matrix as

$$\begin{aligned} n_\sigma &= 1 - \frac{1}{1+e^{-i\alpha_\sigma}U} \\ &= 1 - e^{i\alpha_\sigma}\left[\left(e^{i\alpha_\sigma}-1\right) + (1+U)\right]^{-1}, \end{aligned} \tag{56}$$

and using the Woodbury matrix identity

$$\begin{aligned} &(A+BCD)^{-1} = \\ &\quad A^{-1} - A^{-1}B\left[C^{-1} + DA^{-1}B\right]^{-1}DA^{-1}, \end{aligned} \tag{57}$$

with $B = D = 1$, $C = \left(e^{i\alpha}-1\right)$, and $A = (1+U)$,

$A^{-1} = (1+U)^{-1} = (1-n)$. Thus

$$n_\sigma = 1 - e^{i\alpha_\sigma}(1-n) \times \left\{1 - \left[\frac{1}{e^{i\alpha_\sigma}-1} + (1-n)\right]^{-1}(1-n)\right\}, \quad (58)$$

and we can use batched matrix multiplication, rather than QDR decomposition, to calculate the occupation matrices for each projection angle.

Although we are guaranteed $n_{i,j} \in [0,1]$, the occupation matrices may still be ill conditioned and one may reasonably worry about the stability of multiplying and inverting matrices like $1-n$. However, in practice, we find that the Woodbury method achieves an absolute difference of $\sim 10^{-9}$ compared to the brute force QDR decomposition, even at low temperatures. We use these occupation matrices in momentum and position space to calculate observables in the constrained ensemble.

### B. Calculating the constrained statistical weights

In addition to calculating physical observables from occupation matrices, one must also compute the statistical weights $F[\sigma,\varphi,\theta]$. In Eq. (31b), $F[\sigma,\varphi,\theta]$ is expressed as a ratio of determinants that we expect to be large quantities that are not known with great precision. We therefore simplify the statistical weights as

$$F[\sigma,\varphi,\theta] = e^{i\varphi N}\frac{\det\left[1+e^{-i(\varphi+\theta)}U\right]}{\det[1+U]} \times \frac{\det\left[1+e^{-i(\varphi-\theta)}U\right]}{\det[1+U]} \quad (59)$$

$$= e^{i\varphi N}\frac{\det\left[1+U+\left(e^{-i(\varphi+\theta)}-1\right)U\right]}{\det[1+U]} \times \frac{\det\left[1+U+\left(e^{-i(\varphi-\theta)}-1\right)U\right]}{\det[1+U]}, \quad (60)$$

$$= e^{i\varphi N}\det\left[1+\left(e^{-i(\varphi+\theta)}-1\right)\frac{U}{1+U}\right] \times \det\left[1+\left(e^{-i(\varphi-\theta)}-1\right)\frac{U}{1+U}\right]. \quad (61)$$

## VIII. REDUCING THE NUMBER OF OBSERVABLE CALCULATIONS

Section VII addressed the computation of the $\varphi,\theta$-observables. We then take the discrete Fourier transform of these values to compute the particle projected observables. Suppose we would like to estimate the Fourier integrals in Eq. (29) using $n_f$ points in both $\varphi$ and $\theta$. Since we compute different observables for the $\uparrow$ and $\downarrow$ system, one would naively expect to compute $2n_f^2$ observables. However, we can greatly reduce the number of computed observables.

First, suppose $\varphi_i = -\pi + i2\pi/n_f$ for $i = 0,1,2,\ldots,n_f$ and similarly $\theta_j = -\pi + j2\pi/n_f$ for $j = 0,1,2,\ldots,n_f$. Then we can think of organizing observables in a matrix with rows corresponding to different values of $\varphi$ and columns corresponding to different values of $\theta$. We must then compute observables for all values in the matrices

$$(\varphi+\theta)_{i,j} = -2\pi + (i+j)\frac{2\pi}{n_f}, \quad (62)$$

$$(\varphi-\theta)_{i,j} = (i-j)\frac{2\pi}{n_f}. \quad (63)$$

But note that

$$(\varphi+\theta) = (\varphi-\theta)\,J, \quad (64)$$

where

$$J_{i,j} = \begin{cases}1, & j = n_f - i + 1,\\ 0, & j \neq n_f - i + 1\end{cases}, \quad (65)$$

is the exchange matrix. So if we compute the spin-$\uparrow$ observables, we already have all of the values needed for the spin-$\downarrow$ observables.

This reduces the number of required calculations by a factor of two, but we can do better. Note that the matrix $(\varphi+\theta)_{i,j}$ is a Hankel matrix and therefore has only $2n_f+1$ unique values. For example, with $n_f = 4$, $(\varphi+\theta)_{i,j}$ has the structure

$$\begin{bmatrix} a & b & c & d\\ b & c & d & e\\ c & d & e & f\\ d & e & f & g\end{bmatrix}.$$

So instead of computing observables on the matrix $(\varphi+\theta)_{i,j}$, one can instead compute observables in the array $\omega_k = -2\pi + 4\pi k/(2n_f-1)$ for $k = 0,1,2,\ldots,2n_f-1$. To map the observables back to the independent $\varphi$, $\theta$ space, we use

$$(\varphi+\theta)_{i,j} = \omega_{k=i+j}, \quad (66)$$

$$(\varphi-\theta)_{i,j} = \omega_{k=n_f-1-j+i}, \quad (67)$$

where we assume zero-based indexing in $i$, $j$, and $k$. Thus, we have reduced the number of required observable calculations from $2n_f^2 \to 2n_f - 1$.

## IX. DETERMINING ENERGIES FOR EVEN-ODD STAGGER CALCULATIONS

Measurements of the energy, as well as derived quantities such as the even-odd staggering, are sensitive to lattice effects that must be corrected in order to estimate observables in the continuum limit. In this appendix, we detail the steps required to estimate the energy, and therefore the even-odd energy staggering, in the continuum limit.

Throughout this section, a tilde over a variable will denote that it has been scaled by some other energy scale. We scale energies by the energy of a free Fermi gas at zero temperature, and temperatures and chemical potentials by the Fermi energy. In the text, we will refer to the scaled values as "reduced" and the unscaled values as "absolute."

### A. Extrapolation to the continuum limit

It is instructive to first consider the energy estimation of the free gas of spin-1/2 fermions. In the continuum, one first solves for the reduced chemical potential, $\widetilde{\mu} \equiv \mu/\varepsilon_F$ required to achieve a desired reduced temperature $\widetilde{T} \equiv T/\varepsilon_F$,

$$1 = \frac{3}{2}\widetilde{T}^{3/2} \int_0^\infty \frac{\mathrm{d}z\, z^{1/2}}{1 + \exp\left[z - \widetilde{\mu}/\widetilde{T}\right]}. \tag{68}$$

Once this value of $\widetilde{\mu}$ is determined, it can be used to solve for the reduced energy of a system at temperature $\widetilde{T}$,

$$\widetilde{E}_c \equiv \frac{E_c}{\frac{3}{5}N\varepsilon_F} = \frac{5}{2}\widetilde{T}^{5/2} \int_0^\infty \frac{\mathrm{d}z\, z^{3/2}}{1 + \exp\left[z - \widetilde{\mu}/\widetilde{T}\right]}, \tag{69}$$

where the subscript $c$ indicates that this energy is computed in the continuum.

We can also solve this system on a cubic lattice of side length $L = N_x = N_y = N_z$. The lattice momenta are given by $\vec{p}_n = 2\pi(i_x\hat{x} + i_y\hat{y} + i_z\hat{z})/L$, where $i_j = -L/2+1, \ldots, L/2$, $j \in \{x, y, z\}$. Then, as before, we find the value of the chemical potential required to give us a desired particle number $N$ at the reduced temperature $\widetilde{T}$,

$$N = 2\sum_{\vec{n}} \frac{\alpha \exp\left[-\widetilde{\beta}\frac{\widetilde{p}_{\vec{n}}^2}{2m}\right]}{1 + \alpha \exp\left[-\widetilde{\beta}\frac{\widetilde{p}_{\vec{n}}^2}{2m}\right]}, \tag{70}$$

where the tildes indicate that the lattice momenta and inverse temperature is measured in units of the continuum Fermi energy, $\varepsilon_F = \left(3\pi^2 N/V\right)^{2/3}/2$, and $\alpha \equiv \exp(\beta\mu)$. After determining $\widetilde{\mu}$, one can than calculate the energy of the free Fermi gas on the lattice as

$$\frac{E_\ell}{\varepsilon_F} = 2\sum_{\vec{n}} \frac{\widetilde{p}_{\vec{n}}^2}{2m} \frac{\alpha \exp\left[-\widetilde{\beta}\frac{\widetilde{p}_{\vec{n}}^2}{2m}\right]}{1 + \alpha \exp\left[-\widetilde{\beta}\frac{\widetilde{p}_{\vec{n}}^2}{2m}\right]}, \tag{71}$$

where the subscript $\ell$ indicates that this energy is computed on the lattice.

In Fig. 8, we compare the energies of the free Fermi gas computed on the lattice and in the continuum. For the temperature range of interest $0.1 \leq \widetilde{T} \leq 0.3$, the residual $\delta = |E_c - E_\ell|$ has two zeros at roughly $N \approx 30$ and $N \approx 60$. In typical QMC simulations, one chooses particle numbers in this range to minimize the residuals. However, we constrain our simulations to a range of particle numbers, for which the residuals may not match. To extrapolate to the continuum limit, we multiply our lattice energies by an extrapolation coefficient

$$E_c = C_\ell E_\ell, \quad \text{where} \quad C_\ell \equiv \frac{E_{FFG,c}}{E_{FFG,\ell}}. \tag{72}$$

For the free Fermi gas, Eq. (72) is tautologistic. In our calculations of the interacting gas, applying Eq. (72) amounts to the assumption that the lattice effects predominantly affect the kinetic energy operator as opposed to the potential energy operator. A similar procedure for extrapolating to the continuum limit was used in an AFQMC study of neutron matter with chiral effective field theory [50].

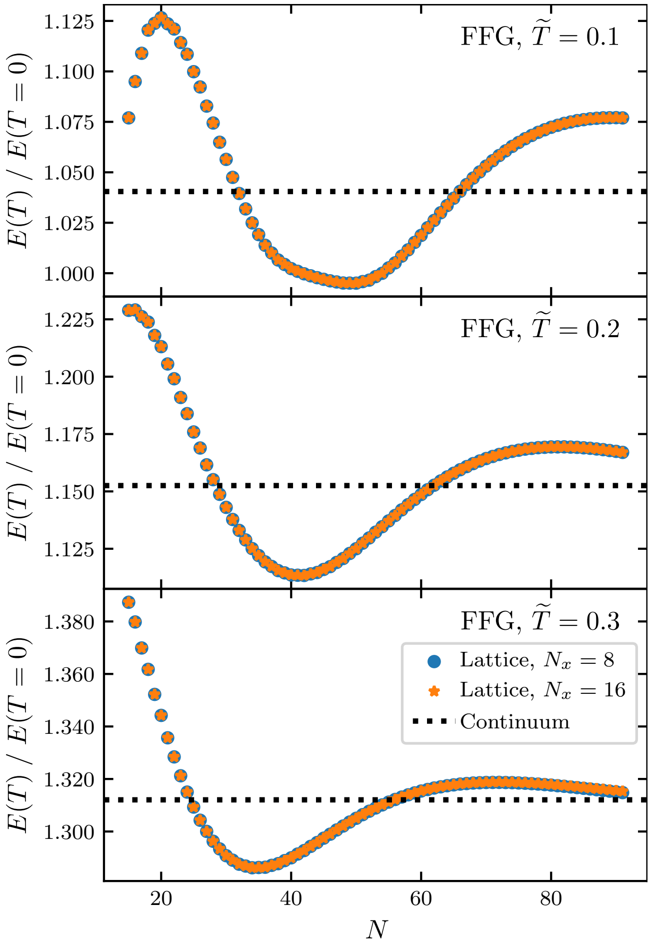


FIG. 8. A comparison of lattice and continuum energies for the free Fermi gas at multiple temperatures: $\widetilde{T} \in \{0.1, 0.2, 0.3\}$ The dashed line indicates the value computed in the continuum, which is independent of particle number. The circles and stars indicate the identical values for an $8^3$ and $16^3$ lattice, respectively.

### B. Finite range correction

In addition to the continuum extrapolation focused on the kinetic energy in Section IX A, we also use the effective range expansion

$$\frac{E}{E_{FFG}} = \xi + \zeta_e k_F r_e + \ldots, \tag{73}$$

where the value of $\zeta_e$ has been estimated as $\zeta_e = 0.12(3)$ [3, 51] and the effective range for a cubic cutoff is [3]

$$r_e = \ell \frac{12\sqrt{2}}{\pi^3} \arcsin \frac{1}{\sqrt{3}} \approx 0.337\ell, \tag{74}$$

where $\ell$ is the lattice constant. We are interested in correcting our lattice calculations conducted with finite effective range to continuum energies with zero range interactions. We therefore combine the continuum limit extrapolation of Section IX A with Eq. (74) by subtracting the finite range correction,

$$\frac{E_c}{E_{FFG}} = C_\ell \frac{E_\ell}{E_{FFG}} - \zeta_e k_F r_e. \tag{75}$$

### C. Reduced temperature shift

The methods of Sections IX A and IX B yield estimates of the energy of a system at some absolute temperature $T$ and particle number $N$. To remove the explicit dependence on particle number, one often scales the energies by the energy of a free Fermi gas at zero temperature and the temperatures by the Fermi energy, as in Eqs. (68) and (69). However, it is important to realize that when estimating observables using the methods in Section II B, the constrained ensemble inherits the absolute temperature of its "parent" GCE simulation. The reduced temperature, $\widetilde{T}$, will be different depending on the projected particle number.

To illustrate this effect, we conducted constrained ensemble simulations of the free Fermi gas. This is computationally inexpensive since, with no interaction term, only one Monte Carlo sample is required to achieve convergence. This allows us to explain the reduced temperature shift inherent in constrained ensemble methods and also serves as a validation step for our simulation software.

In Fig. 9, we show a "stagger plot," similar to Fig. 6 for the unitary Fermi gas. The "parent" GCE simulation was conducted at $\widetilde{T}_{GCE} = 0.2$, from which the constrained ensemble energies were calculated. The blue markers indicate energies calculated using Eq. (72), which are calculated at the same absolute temperature as the GCE,

$$\widetilde{E}\left(N, \widetilde{T}\right) = \widetilde{E}\left(N, \frac{T_{GCE}}{\varepsilon_F(N)}\right). \tag{76}$$

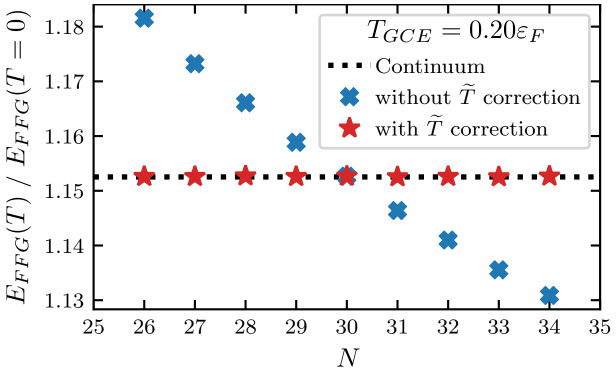


FIG. 9. An energy "stagger" plot for the free Fermi gas, derived using constrained ensembles from a GCE simulation at $\widetilde{T} = T/\varepsilon_F = 0.2$ on a $10^3$ lattice. The energy is scaled by the energy of a free Fermi gas at zero temperature. The dashed line indicates the continuum calculation. The blue 'X' symbols indicate energies calculated at the same absolute temperature as in the GCE, see Eq. (76) whereas the red star symbols indicate energies calculated at the same reduced temperature as in the GCE, see Eq. (77b).

The red markers indicate the energies calculated at the same reduced temperature as in the GCE

$$\widetilde{E}\left(N, \widetilde{T}_{GCE}\right) = \widetilde{E}\left(N, \frac{T_{GCE}}{\varepsilon_F(N)}\right) + f_{\text{shift}}\left(\widetilde{T}_{GCE}, \frac{T_{GCE}}{\varepsilon_F(N)}\right), \tag{77a}$$

where

$$f_{\text{shift}} = \widetilde{E}_{eos}\left(\widetilde{T}_{GCE}\right) - \widetilde{E}_{eos}\left(\frac{T_{GCE}}{\varepsilon_F(N)}\right), \tag{77b}$$

and $\widetilde{E}_{eos}$ is the equation of state of the system under study. For the validation case of the free Fermi gas $\widetilde{E}_{eos} = \widetilde{E}_c$ from Eq. (69). For the interacting gas in our study, we use the equation of state derived from a previous study of the unitary Fermi gas [4]. As expected, the reduced temperature shift brings the red markers in Fig. 9 in line with the continuum value for the same reduced temperature.

Realizing that the constrained ensembles probe different reduced temperatures also allows us to probe many different temperatures from a single GCE simulation. In Fig. 10, we show the results of nine GCE simulations of the free Fermi gas. For each "parent" GCE simulation, we used constrained ensemble methods to calculate energies for nine different particle numbers. Since each of these particle numbers yielded a different reduced temperature, the effect of the constrained ensemble method is to spread each GCE simulation into (sometimes overlapping) temperature ranges.

For reference, we also show the importance of the continuum limit extrapolation in Eq. (72) by plotting the

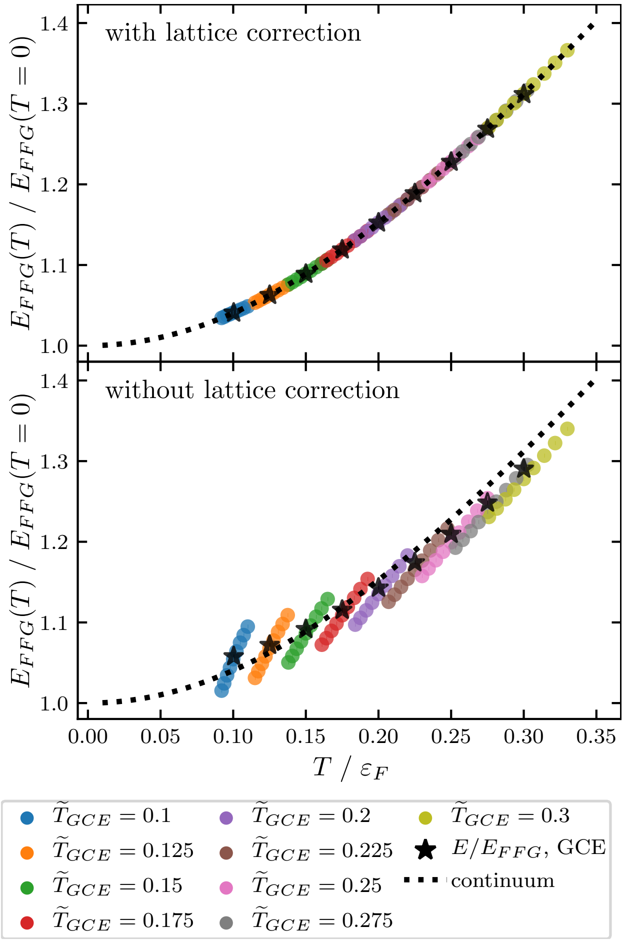


FIG. 10. Constrained ensemble methods "spread" the temperature of each GCE simulation out into sometimes overlapping ranges. Each color in these plots represents one "parent" GCE simulation, the results of which are represented by the black stars. Each GCE simulation is then constrained to a fixed particle number, resulting in different reduced temperatures that spread out away from $\widetilde{T}_{GCE}$.

uncorrected lattice energies (still with reduced temperature shift) in the lower panel of Fig. 10. The behavior is justified when one considers the negative slope of the lattice energies in Fig. 8 around $N \approx 30$ where our GCE calculations were performed. Since an increase in particle number $N$, decreases the reduced temperature $\widetilde{T}$, the residuals in the lower panel of Fig. 10 have the opposite slope to the ones in Fig. 8.

While the continuum limit extrapolation of Section IX A is widely accounted for in AFQMC literature. However, we find no mention of the required reduced temperature corrections in the constrained ensemble literature [17–21]. It is possible that this omission does not affect estimates of the pairing gap since, when evaluating $\Delta_E$ using centered difference formulas, the increase in energy below the central particle number will be approximately cancelled out by the decrease in energy above the central particle number. So in the context of the pairing gap, the temperature correction may be formally required but negligible.

The effect on the spin susceptibility may depend on the way in which it is calculated. In our method, we use the particle asymmetry constrained ensemble so that the scaled spin susceptibility is

$$\frac{\chi_s}{\chi_0} = \frac{2}{3N\widetilde{T}} \sum_{\eta} \eta^2 P(\eta). \tag{78}$$

In this case, each term contributing to the sum comes from a different particle asymmetry projection but the total particle number remains roughly the same so the temperature correction may be safely neglected. Lastly, when directly evaluating energies the temperature correction is plainly required, as demonstrated in Fig. 9.


[1] A. Bulgac, J. E. Drut, and P. Magierski, Phys. Rev. A **78**, 023625 (2008).
[2] A. Bulgac, M. M. Forbes, and P. Magierski, The Unitary Fermi Gas: From Monte Carlo to Density Functionals, in *The BCS–BEC Crossover and the Unitary Fermi Gas*, edited by W. Zwerger (Springer Berlin Heidelberg, Berlin, Heidelberg, 2012) pp. 305–373.
[3] F. Werner and Y. Castin, Phys. Rev. A **86**, 013626 (2012).
[4] J. E. Drut, T. A. Lähde, G. Wlazłowski, and P. Magierski, Phys. Rev. A **85**, 051601 (2012).
[5] S. Jensen, C. N. Gilbreth, and Y. Alhassid, Phys. Rev. Lett. **124**, 090604 (2020).
[6] C. Mora and Y. Castin, Phys. Rev. A **67**, 053615 (2003).
[7] H. F. Trotter, Proceedings of the American Mathematical Society **10**, 545 (1959).
[8] M. Suzuki, Physics Letters A **146**, 319 (1990).
[9] R. Stratonovich, in *Soviet Physics Doklady*, Vol. 2 (1957) p. 416.
[10] J. Hubbard, Phys. Rev. Lett. **3**, 77 (1959).
[11] J. E. Hirsch, Phys. Rev. B **28**, 4059 (1983).
[12] N. Metropolis, A. W. Rosenbluth, M. N. Rosenbluth, A. H. Teller, and E. Teller, The Journal of Chemical Physics **21**, 1087 (1953).
[13] W. K. Hastings, Biometrika **57**, 97 (1970).
[14] C. Gilbreth and Y. Alhassid, Computer Physics Communications **188**, 1 (2015).
[15] A. Gelman and D. B. Rubin, Statist. Sci. **7**, 457 (1992).
[16] S. P. Brooks and A. Gelman, Journal of Computational and Graphical Statistics **7**, 434 (1998).
[17] W. E. Ormand, D. J. Dean, C. W. Johnson, G. H. Lang, and S. E. Koonin, Phys. Rev. C **49**, 1422 (1994).
[18] K. Langanke, D. J. Dean, P. B. Radha, Y. Alhassid, and S. E. Koonin, Phys. Rev. C **52**, 718 (1995).

[19] C. N. Gilbreth and Y. Alhassid, Phys. Rev. A **88**, 063643 (2013).
[20] S. Jensen, C. Gilbreth, and Y. Alhassid, The European Physical Journal Special Topics **227**, 2241 (2019).
[21] A. Bulgac, Phys. Rev. C **100**, 034612 (2019).
[22] J. Braun, J.-W. Chen, J. Deng, J. E. Drut, B. Friman, C.-T. Ma, and Y.-D. Tsai, Phys. Rev. Lett. **110**, 130404 (2013).
[23] A. C. Loheac, J. Braun, and J. E. Drut, Phys. Rev. D **98**, 054507 (2018).
[24] A. C. Loheac, J. Braun, J. E. Drut, and D. Roscher, Phys. Rev. A **92**, 063609 (2015).
[25] L. Rammelmüller, W. J. Porter, J. E. Drut, and J. Braun, Phys. Rev. D **96**, 094506 (2017).
[26] J. Braun, J. E. Drut, and D. Roscher, Phys. Rev. Lett. **114**, 050404 (2015).
[27] D. Roscher, J. Braun, J.-W. Chen, and J. E. Drut, Journal of Physics G: Nuclear and Particle Physics **41**, 055110 (2014).
[28] B. Mukherjee, P. B. Patel, Z. Yan, R. J. Fletcher, J. Struck, and M. W. Zwierlein, Phys. Rev. Lett. **122**, 203402 (2019).
[29] C. Carcy, S. Hoinka, M. G. Lingham, P. Dyke, C. C. N. Kuhn, H. Hu, and C. J. Vale, Phys. Rev. Lett. **122**, 203401 (2019).
[30] J. E. Drut, Phys. Rev. A **86**, 013604 (2012).
[31] R. Rossi, T. Ohgoe, E. Kozik, N. Prokof'ev, B. Svistunov, K. Van Houcke, and F. Werner, Phys. Rev. Lett. **121**, 130406 (2018).
[32] S. Jensen, C. N. Gilbreth, and Y. Alhassid, The contact in the unitary Fermi gas across the superfluid phase transition (2019), arXiv:1906.10117 [cond-mat.quant-gas].
[33] S. Tan, Annals of Physics **323**, 2952 (2008).
[34] S. Tan, Annals of Physics **323**, 2971 (2008).
[35] S. Tan, Annals of Physics **323**, 2987 (2008).
[36] E. Braaten, Universal Relations for Fermions with Large Scattering Length, in *The BCS–BEC Crossover and the Unitary Fermi Gas*, edited by W. Zwerger (Springer Berlin Heidelberg, Berlin, Heidelberg, 2012) pp. 193–231.
[37] P. Pieri, A. Perali, and G. C. Strinati, Nature Physics **5**, 736 (2009).
[38] E. Burovski, E. Kozik, N. Prokof'ev, B. Svistunov, and M. Troyer, Phys. Rev. Lett. **101**, 090402 (2008).
[39] P. Magierski, G. Wlazłowski, and A. Bulgac, Phys. Rev. Lett. **107**, 145304 (2011).
[40] M. N. Barber, Finite-size scaling in phase transitions and critical phenomena, in *Phase Transitions and Critical Phenomena*, Vol. 8, edited by C. Domb and J. Lebowitz (Academic Press, 1983) p. 146.
[41] J. Carlson, S.-Y. Chang, V. R. Pandharipande, and K. E. Schmidt, Phys. Rev. Lett. **91**, 050401 (2003).
[42] S. Y. Chang, V. R. Pandharipande, J. Carlson, and K. E. Schmidt, Phys. Rev. A **70**, 043602 (2004).
[43] L. Neufcourt, Y. Cao, W. Nazarewicz, and F. Viens, Phys. Rev. C **98**, 034318 (2018); L. Neufcourt, Y. Cao, S. A. Giuliani, W. Nazarewicz, E. Olsen, and O. B. Tarasov, Quantified limits of the nuclear landscape (2020), arXiv:2001.05924 [nucl-th]; L. Neufcourt, Y. Cao, S. Giuliani, W. Nazarewicz, E. Olsen, and O. B. Tarasov, Phys. Rev. C **101**, 014319 (2020).
[44] S. Wesolowski, R. J. Furnstahl, J. A. Melendez, and D. R. Phillips, Journal of Physics G: Nuclear and Particle Physics **46**, 045102 (2019).
[45] T. Hastie, R. Tibshirani, and J. Friedman, Model Assessment and Selection, in *The Elements of Statistical Learning: Data Mining, Inference, and Prediction* (Springer New York, New York, NY, 2009) pp. 219–259.
[46] C. K. Williams and C. E. Rasmussen, *Gaussian Processes for Machine Learning*, Vol. 2 (MIT press Cambridge, MA, 2006).
[47] See D. Duvenaud, *Automatic model construction with Gaussian processes*, Ph.D. thesis, University of Cambridge (2014) for practical advice on choosing covariance functions.
[48] F. Pedregosa, G. Varoquaux, A. Gramfort, V. Michel, B. Thirion, O. Grisel, M. Blondel, P. Prettenhofer, R. Weiss, V. Dubourg, J. Vanderplas, A. Passos, D. Cournapeau, M. Brucher, M. Perrot, and E. Duchesnay, Journal of Machine Learning Research **12**, 2825 (2011).
[49] P. Virtanen, R. Gommers, T. E. Oliphant, M. Haberland, T. Reddy, D. Cournapeau, E. Burovski, P. Peterson, W. Weckesser, J. Bright, S. J. van der Walt, M. Brett, J. Wilson, K. Jarrod Millman, N. Mayorov, A. R. J. Nelson, E. Jones, R. Kern, E. Larson, C. Carey, İ. Polat, Y. Feng, E. W. Moore, J. Vand erPlas, D. Laxalde, J. Perktold, R. Cimrman, I. Henriksen, E. A. Quintero, C. R. Harris, A. M. Archibald, A. H. Ribeiro, F. Pedregosa, P. van Mulbregt, and S. . . Contributors, Nature Methods **17**, 261 (2020).
[50] G. Wlazłowski, J. W. Holt, S. Moroz, A. Bulgac, and K. J. Roche, Phys. Rev. Lett. **113**, 182503 (2014).
[51] J. Carlson, S. Gandolfi, K. E. Schmidt, and S. Zhang, Phys. Rev. A **84**, 061602 (2011).
